# Supplementary material for: Topological Thermoelectricity in Metals
Source: arXiv:1806.11406 source file (2018-07-02)
Supplement: Supplementary file 1 [file SI_arxiv-compressed.pdf]

# Supplemental Information: Topological Thermoelectricity in Metals


Sobhit Singh,[1] QuanSheng Wu,[2,3,*] Changming Yue,[4] Aldo H. Romero,[1] and Alexey A. Soluyanov[3,5,6]

[1] *Department of Physics and Astronomy, West Virginia University, Morgantown, WV-26505-6315, USA*

[2] *Institute of Theoretical Physics, Ecole Polytechnique Fédérale de Lausanne (EPFL), CH-1015 Lausanne, Switzerland*

[3] *Theoretical Physics and Station Q Zurich, ETH Zurich, CH-8093 Zurich, Switzerland*

[4] *Beijing National Laboratory for Condensed Matter Physics, and Institute of Physics, Chinese Academy of Science, Beijing 100190, China*

[5] *Physik-Institut, Universität Zürich, Winterthurerstrasse 190, CH-8057 Zurich, Switzerland*

[6] *Department of Physics, St. Petersburg State University, St. Petersburg, 199034, Russia*



(Dated: June 29, 2018)


This supplemental information (SI) file contains results of our work that are not included in the main text. In particular, here we provide the optimized lattice parameters, electronic band structures, electronic density of states (DOS), phonon spectrum and atom projected phonon DOS for all the studied materials. In addition, we illustrate the surface electronic structure, surface phonon spectrum, thermoelectric properties and results of crystal stability and elastic properties of the predicted TaSb compound. We also demonstrate the mechanism of the topological phonon band-crossing in materials hosting triply-degenerate points (TDP) in their phonon spectrum. Finally, we give the full description of methodology used to perform all the presented simulations.

TABLE I: Considered atomic masses (in $g/mol$ units) of different atoms

| Ta | Nb | N | P | As | Sb | Bi | Ti | Zr | Hf | S | Se | Te |
|---|---|---|---|---|---|---|---|---|---|---|---|---|
| 180.95 | 92.91 | 14.01 | 30.97 | 74.92 | 121.8 | 209.0 | 47.90 | 91.22 | 178.49 | 32.06 | 78.96 | 127.60 |

---


*S. Singh and Q. Wu equally contributed to this work

TABLE II: Optimized lattice parameters (in Å) and the presence of non-trivial topology of electron and phonon spectra for TaX and NbX ($X$ = N, P, As, Sb, Bi) family compounds. All structures listed below were considered to have $P\bar{6}m2$ (187) space group of the crystal structure.

| Composition | Optimized lattice parameters | Topological features in the electron spectrum | Topological features in the phonon spectrum |
|---|---|---|---|
| TaN | a = b = 2.946, c = 2.894 | Yes (Fig. 9) | No (Fig. 17) |
| TaP | a = b = 3.313, c = 3.339 | Yes (Fig. 10) | No (Fig. 18) |
| TaAs | a = b = 3.407, c = 3.487 | Yes (Fig. 11) | No (Fig. 19) |
| TaSb | a = b = 3.584, c = 3.807 | Yes (Fig 2) | Yes (Fig. 8) |
| TaBi | a = b = 3.658, c = 3.964 | Yes (Fig. 12) | Yes (Fig. 20) |
| NbN | a = b = 2.976, c = 2.901 | Yes (Fig. 13) | No (Fig. 21) |
| NbP | a = b = 3.333, c = 3.359 | Yes (Fig. 14) | No (Fig. 22) |
| NbSb | a = b = 3.714, c = 3.714 | Yes (Fig. 15) | No (Fig. 23) |
| NbBi | a = b = 3.678, c = 3.963 | Yes (Fig. 16) | No (Fig. 24) |

## I. CRYSTAL STRUCTURE AND STABILITY OF TaSb

Fig. 1(a-b) shows the crystal structure of TaSb compound in $P\bar{6}m2$ space group (no. 187). Lattice parameters of the optimized cell are: $a = b = 3.584$ Å, $c = 3.807$ Å. The Ta-Sb bond length is 2.81 Å. This structure was obtained by performing a systematic structural search on Ta-Sb binaries using the Minima Hopping Method (MHM) [1, 2]. The MHM utilizes an efficient dynamical algorithm to explore the potential energy surface (PES) of a given composition by performing short molecular dynamics (MD) simulations. The MD escape moves help to overcome minima, moving to different minima. To improve the efficiency of each escape move, the initial atom velocities of the MD simulations are aligned along the soft-mode directions. Here we utilize random Boltzmann velocity distribution to add a kinetic energy ($E_{kin}$) in order to assist the searcher to overcome the energy barrier ($E_{barrier}$) between two neighboring local minima and escape the local minimum. Generally, we start with a small $E_{kin}$ and make an attempt to escape the local minimum, if the searcher manages to escape the $E_{barrier}$ (*i.e.* $E_{kin} > E_{barrier}$), MD step stops. Otherwise, algorithm increases $E_{kin}$ with an aim to cross the $E_{barrier}$. The algorithm also stores the history of the visited local minima. If the searcher lands into a local minima (after MD escape move) that has already been visited, the algorithm further increases the $E_{kin}$ with aim to find a new local minima. Thus, $E_{barrier}$ is continuously adjusted during the MD simulations. The MHM exploits the Bell-Evans-Polanyi (BEP) principle [3] to determine the direction of forces on atoms (*i.e.* velocities) required for the MD escape move. According to this principle, it is more likely to find a lower energy local minimum if we align the MD escape move in such a way that searcher crosses the energy barrier through a soft mode direction. The soft mode direction can be determined from the Hessian matrix. The algorithm aligns the velocity vectors on each atom during the MD escape move along the direction which corresponds to the Hessian eigen vector with lowest Hessian eigen value. This ensures that the searcher is crossing the $E_{barrier}$ through a soft mode direction [4]. Once a new local minima is obtained, the MD step stops and geometrical optimization is performed with tighter convergence parameters.

This method has been proven to remarkable predict not only the new crystal structures of a wide range of materials but it has also recovered the previously known phases of a given composition [1, 2, 5–7]. More details of the MHM calculations can be found in Refs. [2, 6]. After performing an extensive exploration of the PES of TaSb (each time starting from a different initial configuration on the phase space) we found the $P\bar{6}m2$ structure as the global minima with the lowest formation energy. In fact, the same $P\bar{6}m2$ structure has been experimentally reported to be the ground state structure of other compounds of this family [8–11].

Since the proposed structure is new and has not been experimentally synthesized yet, it is important to check its stability using different numerical techniques. The absence of imaginary phonon frequencies in the calculated phonon spectrum at 0 K (shown in the main file) and at 300 K (Fig. 1(d)) supports the thermodynamical stability of this compound at 0 K as well as at room temperature.

To test the mechanical stability of TaSb, we calculate the elastic properties using the stress-strain relations as implemented in VASP *ab-initio* code [12, 13]. The elastic constants ($C_{ij}$) were converged to less than 1.0 GPa with the 15×15×15 $k$-mesh. Spin-orbit coupling (SOC) was included in the calculation of elastic constants. The noteworthy elastic constants [14, 15] for TaSb hexagonal system are: $C_{11}$ = 176.5 GPa, $C_{12}$ = 77.2 GPa, $C_{13}$ = 124.5 GPa, $C_{33}$ = 264.2 GPa, and $C_{44}$ = 141.7 GPa. It is well know that a crystal is mechanically stable if it satisfies the Born-Huang elastic stability criterion [16]. In particular, for a hexagonal system the conditions for mechanical stability [14, 17]

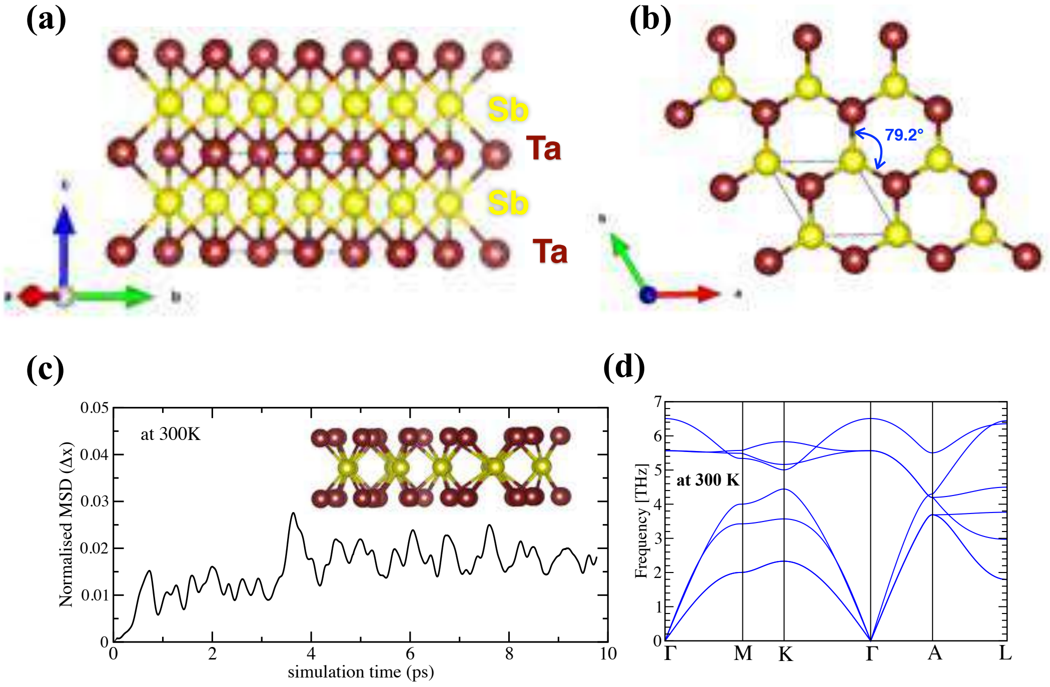


FIG. 1: (Color online) Figure (a) and (b) shows the top and side views of the crystal structure of TaSb compound in $P\bar{6}m2$ space group, respectively. Ta atoms (maroon color) occupy the (2/3, 0.0, 2/3) site, and Sb atoms (golden color) occupy the (0.0, 1/2, 0.0) site. (c) Figure represents change in the average mean-square displacement (MSD) as a function of the simulation time (in ps) at 300 K. To illustrate the quantitative change in MSD, we have normalized MSD over the total Ta-Sb bond length. The inset of Figure (c) shows the geometric structure obtained at the end of MD simulations. (d) Phonon bandstructure calculated at 300 K.

are: $C_{11} - |C_{12}| > 0$, $(C_{11} + 2C_{12})C_{33} - 2C_{13}^2 > 0$, and $C_{44} > 0$, with the above listed values of $C_{11}$, $C_{12}$ , $C_{13}$, $C_{14}$, $C_{33}$, and $C_{44}$. According to the calculated elastic constants values, TaSb compound satisfies the mechanical stability criteria for the hexagonal unit cell, thus confirming the mechanical stability of TaSb in $P\bar{6}m2$ crystal structure. We also evaluate the bulk modulus (B), shear modulus (G), Young's modulus (E) and Poisson's ratio ($v$) for TaSb by using the Voigt-Reuss-Hill approximation [18]. The average values we found are: B $\sim$ 134 GPa, G $\sim$ 75 GPa, E $\sim$ 190 GPa, and $v = 0.27$. The B/G ratio classifies materials according to their brittleness or ductileness [19]. If B/G $<$ 1.75, a material behaves as a brittle material, while B/G $>$ 1.75 corresponds to a ductile material [7]. Based on the calculated B/G ratio (= 1.8), we classify TaSb as a ductile material. Notably, all six eigenvalues of elastic stiffness tensor and elastic moduli are positive which further support the mechanical stability of this compound.

In order to assess the thermal stability of TaSb at room temperature, we perform MD simulations at 300 K for a supercell of size $4 \times 4 \times 4$. Fig. 1(c) shows the average mean-square displacement (MSD) of atoms as a function of MD simulation time. The maximum amplitude of MSD is very small ($< 3\%$) compared to the Ta-Sb bond length. Additionally, one can notice that the geometric structures at 0 K [Fig. 1(a)] and at 300 K [inset of Fig. 1(c)] are quite similar, confirming the stability of the studied structure at room temperature. Phonons calculated at 300 K using the temperature dependent effective potential (TDEP) method, discussed in the methodology section, exhibit no imaginary frequency. Thus, our results imply that the TaSb structure is stable and we believe that it can be experimentally synthesized under suitable ambient conditions. In fact, other similar compositions Ta$X$, Nb$X$ ($X$ = N, P, As) have already been experimentally realized [8–11]. The possibility to observe topology-driven physics in this structure motivates us to thoroughly investigate its electronic and vibrational properties.

## II. ELECTRONIC BAND STRUCTURE OF TaSb

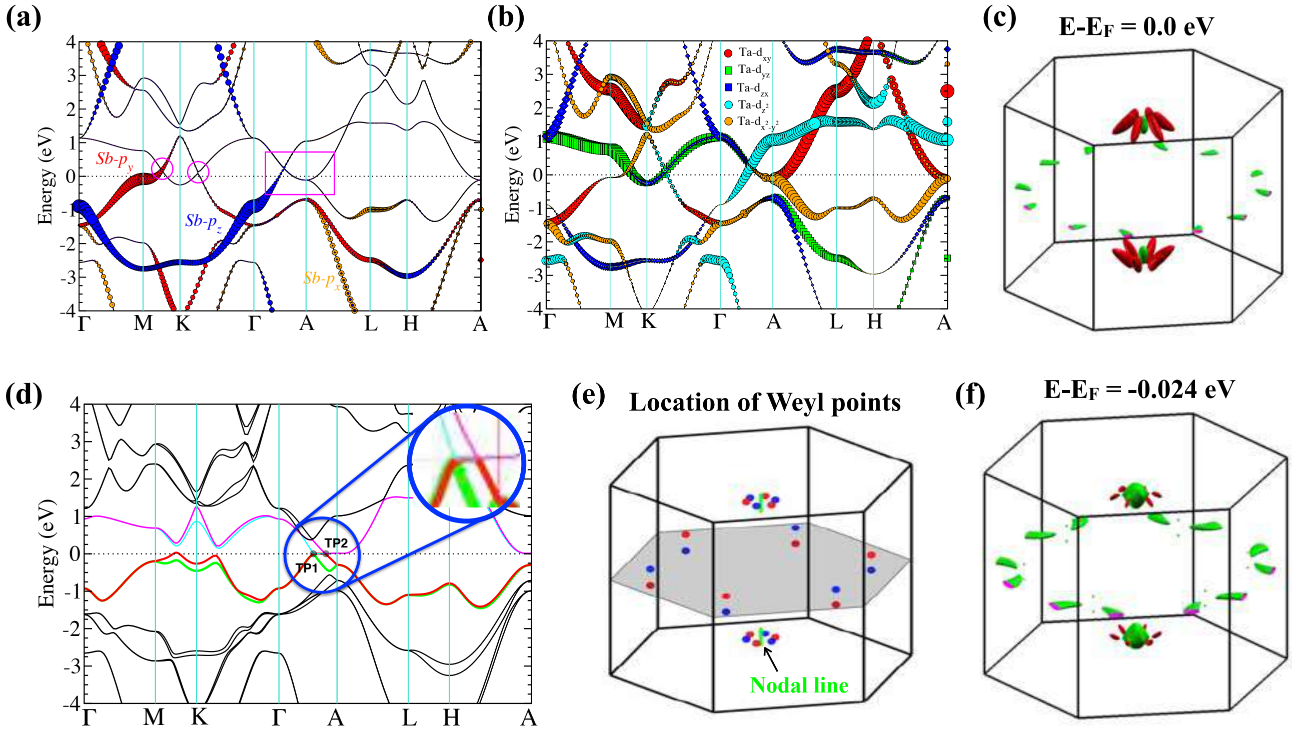


FIG. 2: (Color online) Figures (a-b) represent the electronic band structure calculated without inclusion of SOC. Projection of the Sb-$p$ atomic orbitals is shown in panel (a) while projection of Ta-$d$ orbitals is shown in panel (b). The magenta circles mark the location of points that belong to a Dirac nodal line centered at K-point, and magenta rectangles depicts the location of gapless nodal line present along the $\Gamma - A$ path. Panel (d) represents the electronic band structure calculated with-SOC. The inset of panel (d) shows the enlarged view of the gapless nodal line. The locations of triple-points (TP1 and TP2) at the end of the gapless nodal line are marked by black circles. For better visibility, bands near the Fermi-level are plotted in different colors. Location of all the Weyl points present in the Brillouin zone is shown in panel (e) (For their exact locations, see Tab. III). Red (blue) spheres denote the Weyl points having positive (negative) chirality. The green lines mark the location of the gapless nodal line. Six pairs of Weyl points that appear in the shaded $k_x - k_y$ plane are of type-I, while the other six pairs of Weyl points that surround the gapless nodal line are of type-II. Panels (c) and (f) show the Fermi-surface calculated at $E - E_F$ = 0.0 eV and $E - E_F$ = -0.024 eV, respectively. One can observe the formation of type-II Weyl points as touching points of electron and hole pockets along the $\Gamma - A$ path.

The electronic band structure of TaSb, calculated along the high symmetry directions of the BZ with SOC, is shown in Fig. 2(d). Figs. 2(a-b) represent the Sb and Ta orbitals projected fat bands calculated in absence of SOC. Fig. 2(a) indicates that Sb–5$p_y$ and Sb–5$p_z$ orbitals compose only the valence band states near the Fermi-level, whereas, the Ta-3$d$ orbitals predominantly contribute to both the conduction and the valence bands [see Fig. 2b)]. One can notice the presence of two evenly dispersed gapless points near the Fermi-level, marked by magenta circles in Fig. 2(a), along the $M - K$ and $K - \Gamma$ directions. A further analysis of the electronic band structure near K-point reveals that these gapless points belong to a Dirac nodal line centered at the K-point. This Dirac nodal line primarily appears due to the

inverted band ordering of Ta–$d_{x^2-y^2}$ and Ta–$d_{yz+zx}$ orbitals near K-point [see Fig. 2(d)]. Additionally, the inverted band ordering of multiple Ta–$d$ orbitals along the $\Gamma - A$ direction yields another four-fold degenerate gapless nodal line (marked by a magenta rectangle). This nodal line is protected by the $C_{3v}$ rotational symmetry of the crystal and it is composed of Ta–$d_{z^2}$, $d_{x^2-y^2}$, $d_{zx}$, $d_{xy}$ orbitals.

In presence of SOC, the spin-degeneracy of electronic bands is lost except at the time-reversal-invariant-momenta (TRIM) points. The Dirac nodal line surrounding the K-point disappears and an energy gap opens along the $M-K-\Gamma$ path [Fig. 2(d)]. The SOC induced energy gap is about $\sim$ 0.18 eV at this point, due to the large SOC of Ta and Sb atoms. A careful analysis of the bands away from the high-symmetry direction manifests that the gapless Dirac nodal line breaks into pairs of gapless Weyl points located at the same energy near the K-point. These pairs of Weyl points share opposite topological charge and they feature a source and a sink of Berry curvature in momentum space. These Weyl points are of type-I and have already been discovered in experiments [20–22]. Although, SOC breaks the Dirac nodal line into type-I Weyl points, it does not destroy the gapless nodal line along $\Gamma - A$ completely. However, SOC partially lifts the degeneracy of the gapless nodal line from the four-fold to the two-fold. It is note worthy that the gapless nodal line lies exactly at the Fermi-level. Two triply-degenerate gapless nodal points appear at the ends of the nodal line as depicted in Fig. 2(d). These gapless points, known as triple-points, emerge at the touching point of three bands (two valence and one conduction bands) near the Fermi-level as shown in the inset of Fig. 2(e) and are protected by the $C_{3v}$ rotational symmetry and vertical mirror symmetries of the crystal [23]. The exact location of the triple-points along $\Gamma - A$ path is: TP1 (0, 0, 0.298 $\frac{2\pi}{c}$) and TP2 (0, 0, 0.398 $\frac{2\pi}{c}$).

The existence of three-component fermions has been recently confirmed by angle-resolved photoemission spectroscopic (ARPES) measurements on MoP crystals [24]. The work of ref. [23] predicted the existence of two topologically distinct types of triple-point-metals (type A and type B). These two types can be easily classified by looking at the crystal symmetry of system and the total number of accompanying nodal lines. The conditions for the appearance of the two types of triple-point fermions, the topological differences between them, and a list of hosting space groups are given in detail in Ref. [23]. All the Ta$X$ and Nb$X$ ($X$ = P, N, As) family compounds having $P\bar{6}m2$ space group host topologically protected type-A triple-point fermions, connected by a single nodal line.

Although there is no clear signature of Weyl points near the gapless nodal line and the triple-points in Fig. 2(d), previous works reported the presence of type-II Weyl points near such gapless nodal lines [23, 25]. Therefore, to pin down the location and chirality of all Weyl points, we perform a comprehensive analysis of the electronic structure near the Fermi-level. We evaluate the energy gap ($\Delta E$) between the $N^{th}$ and $(N+1)^{th}$ bands in the 3D BZ; i.e. $\Delta E = E(N+1) - E(N)$. Here, $N$ is the total number of occupied bands. Such obtained gapless points mark the location of Weyl points, and the obtained gapless line is a representative of the nodal line in BZ. We further integrate the Berry curvature in a small sphere enclosing each individual Weyl points, and thus we calculate the topological charge of each Weyl point [26, 27]. Fig. 2(e) shows the location and topological charge of all Weyl points. We observe that six-pairs of type-I Weyl points appear near $k_z = 0$ plane at $E - E_F$ = -0.007 eV energy. The exact location of a pair of Weyl points close to the K-point is (according to the tight-binding calculations): (0.486$\frac{2\pi}{a}$, -0.243$\frac{2\pi}{b}$, $\pm$ 0.0421$\frac{2\pi}{c}$). We also observe two gapless nodal lines (marked by green color) connecting the triple-points TP1 and TP2 in the full BZ. Surprisingly, we discover three additional pairs of Weyl points located near each gapless nodal line. These Weyl points appear at $k_z = \pm$ 0.357 ($\frac{2\pi}{c}$) near $E - E_F$ = -0.024 eV energy. The energy band dispersion near these Weyl points suggests that these Weyl points have type-II character [28]. The type-II Weyl fermions appear

at the touching points of the electron and hole pockets in reciprocal space, which happens due to the tilted linear dispersion of spin non-degenerate bands near Fermi-level.

We illustrate the evolution of the Fermi-surface calculated at different energy values in Fig. 2(c,f). We can evidently observe the formation of both type-I and type-II Weyl points in the Fermi-surface plots. Six type-I Weyl points are near $k_z = 0$ plane, and six type-II Weyl points are located near the gapless nodal line. The touching of electron and hole pockets forming six isolated type-II Weyl points can be clearly noticed.

TABLE III: Coordinates of Weyl points and triple-points (TP) present in TaSb.

| | Coordinates |
|---|---|
| Triple-points (TP) | TP1 (0.0, 0.0, $\pm 0.298 \frac{2\pi}{c}$ ) |
| | TP2 (0.0, 0.0, $\pm 0.398 \frac{2\pi}{c}$ ) |
| Weyl-points (type-I) near K | ($0.486 \frac{2\pi}{a}$, $-0.243 \frac{2\pi}{b}$, $\pm\ 0.0421 \frac{2\pi}{c}$) |
| Weyl-points (type-II) near TP | ($\pm 0.034 \frac{2\pi}{a}$, $\pm 0.034 \frac{2\pi}{b}$, $\pm\ 0.357 \frac{2\pi}{c}$) |
| | ($\pm 0.06 \frac{2\pi}{a}$, 0.00, $\pm\ 0.357 \frac{2\pi}{c}$) |

## III. TOPOLOGICAL ELECTRONIC SURFACE BAND STRUCTURE OF TaSb

The presence of Weyl points in the bulk suggests the existence of ARPES-observable open Fermi-arcs at the surface of Weyl semimetals [29]. Therefore, we study the topological features of surface states by means of the tight binding model constructed using the maximally localized Wannier functions (MLWF) method [30, 31], using WannierTools software [26]. The results for different terminations of (100) and (001) surfaces are presented in Fig. 3 and Fig. 4, respectively. The positive and the negative Weyl points project themselves onto each other on the (001) surface, and thus making the Fermi-arc invisible on the (001) surface of BZ. Therefore, we focus our attention on the (100) surface where the projected Weyl points do not neutralize their non-trivial features. Fig. 3(a) shows the projection of all Weyl points and nodal lines on the (100) surface of BZ. The surface electronic bandstructure calculated for Sb and Ta terminated (100) surfaces are shown in Fig. 3(d) and Fig. 3(e), respectively. The electronic bandstructures for Ta and Sb terminated surfaces are not identical due to the broken inversion symmetry at the surface. The gapless surface states, connecting the bulk valence bands to the bulk conduction bands, can be observed in both surface bandstructure plots [Fig. 3(d-e)]. These gapless surface states feature themselves as open Fermi-arcs connecting opposite Weyl points on the (100) surface [see Fig. 3(f-i)]. Since the Weyl points are well dispersed on the (100) surface, the connecting Fermi-arcs are quite long in momentum space which makes them accessible in ARPES measurements.

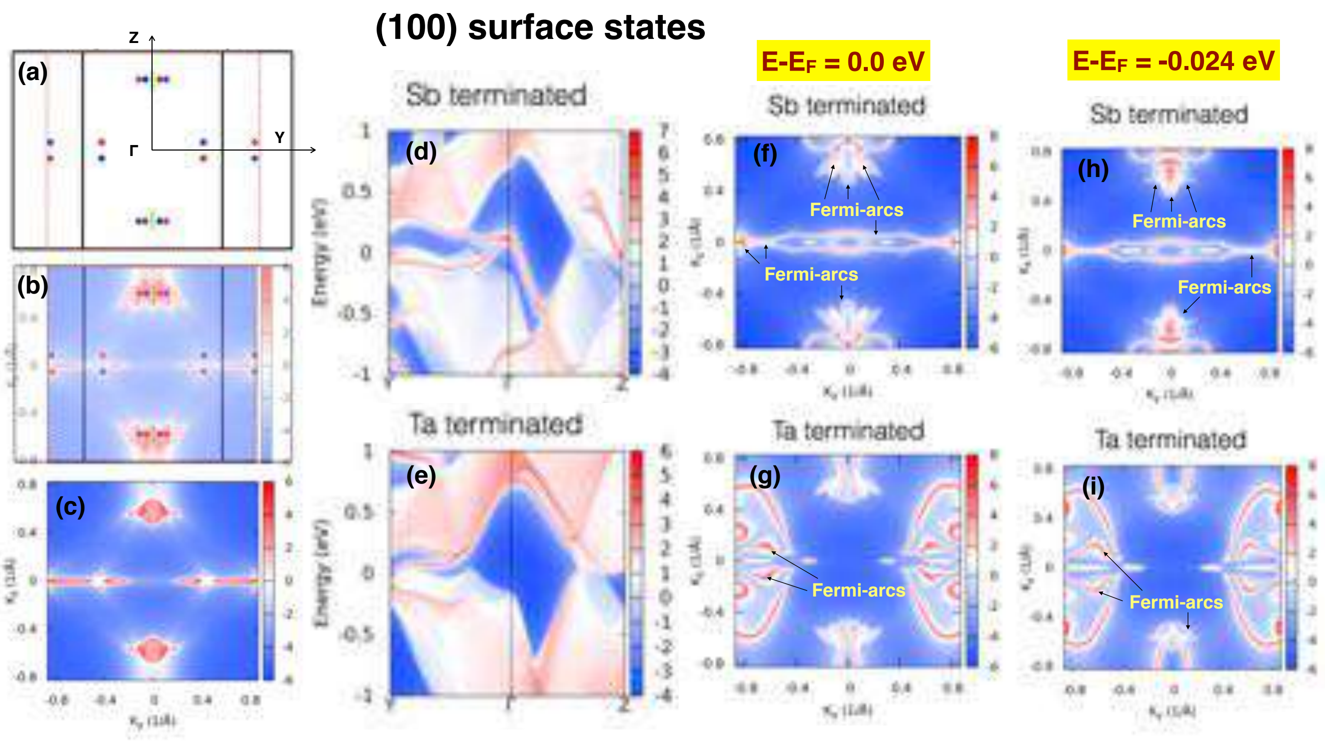


FIG. 3: (Color online) Electronic structure of (100) surface with two possible surface terminations: (a) Distribution of the projected Weyl points on the (100) surface. Red (blue) spheres denote the Weyl points having positive (negative) topological charge. Projection of the Ta-terminated (b) and Sb-terminated (c) surface density of states. Figures (d) and (e) represent the calculated electronic bandstructure for Ta and Sb terminated (100) surfaces, respectively. Figures (f-i) show the Fermi-surface calculated at $E - E_F$ = 0.0 eV (f, g) and $E - E_F$ = -0.024 eV (h, i), clearly demonstrating the location of Fermi-arcs on the Ta and Sb terminated (100) surfaces, respectively.

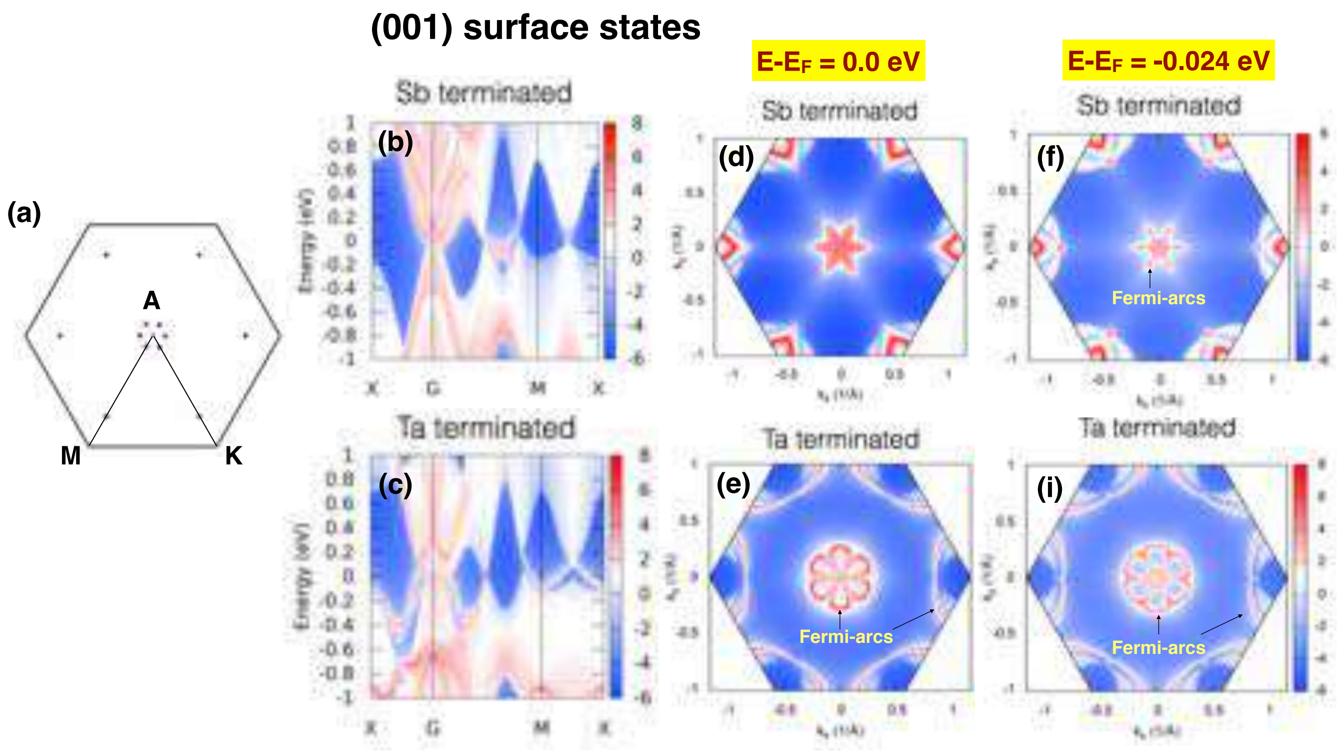


FIG. 4: (Color online) Electronic structure of (001) surface with two possible surface terminations: (a) Distribution of the projected Weyl points on the (001) surface. Red (blue) spheres denote the Weyl points having positive (negative) topological charge. Figures (b) and (c) represent the calculated electronic bandstructure for Ta and Sb terminated (100) surfaces, respectively. Figures (d-i) demonstrate the Fermi-arcs on the Ta and Sb terminated (100) surfaces, respectively.

## IV. TOPOLOGICAL PHONONS IN TaSb

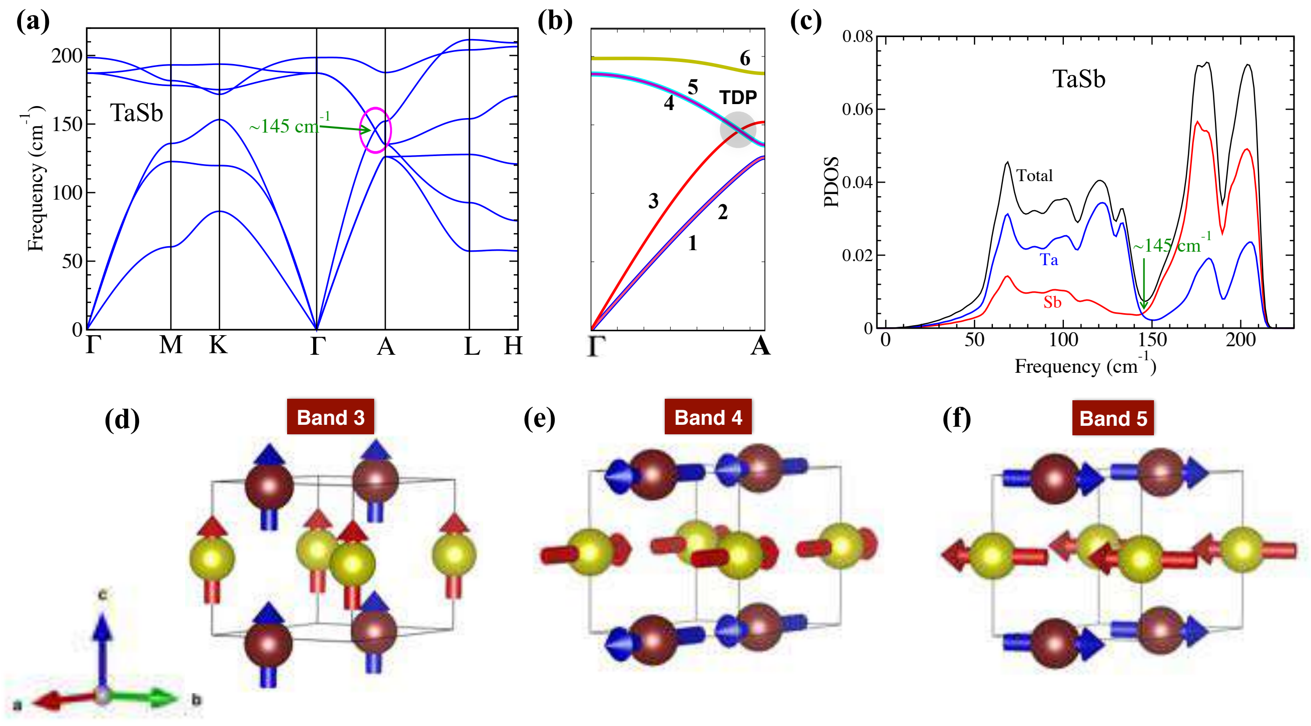


FIG. 5: (Color online) (a) The calculated phonon bandstructure of bulk TaSb. (b) The phonon bandstructure calculated along the $\Gamma - A$ path. Each color depicts a particular phonon eigen vector and the numbers are label to each phonon bands. The phonon bands 4 and 5 are degenerate along the $\Gamma - A$ path. The triple-degenerate point (TDP) is highlighted by a black circle. (c) Atom projected phonon density of states (PDOS) for bulk TaSb. Red color corresponds to the Ta atom while blue color corresponds to the Sb atom. Figures (d-f) are the schematic representations of the vibration of atoms corresponding to the 3rd, 4th and 5th phonon bands (normal modes) at a q-point located between the Γ and TDP point.

The atom-projected phonon density of states (PDOS) and phonon spectrum of TaSb calculated along the high symmetry directions of BZ are shown in Figure 5. We observe that one acoustic branch (no. 3) and two degenerate optical branches (no. 4 and 5) intersect each other along the $\Gamma - A$ path forming a gapless triple-degenerate-point (TDP) as marked in Figure 5(b). To rule out the possibility of artifacts in the plotting, we analyze the polarization of each phonon eigen vector along the $\Gamma - A$ path calculated using a very dense $q$-mesh. Our results remarkably confirm that the phonon band-crossing at TDP is real. The TDP is located at frequency 145 $\mathrm{cm}^{-1}$ and at (0, 0, 0.428) $q$-point. A phonon band-inversion can be noticed above the TDP, where two degenerate optical modes (no. 4 and 5 unusually attain lower frequency than the acoustic mode (no. 3). The phonon band-inversion, at the high-symmetry point A(0, 0, $\frac{\pi}{c}$), is indicative of the non-trivial topological nature of the vibrational properties in TaSb compound. It is worth to mention that this phonon band-inversion along $\Gamma - A$ path is missing for the case of other triple-point-metals (except TaBi), even though all triple-point-metals share isoelectronic properties. One main reason of the existence of phonon band-inversion is the fact that the atoms of almost equal masses constitute the TaSb and TaBi compounds. When there is a significant difference in the mass of the constituent atoms, the above-mentioned phonon band-crossing does not take place and a wide frequency gap appears in the phonon spectrum.

Figure 5 (d-f) represents the nature of the atomic vibrations corresponding to each phonon eigen mode near the TDP. The 3rd phonon band corresponds to the acoustic (in-phase) vibration of Ta and Sb atoms oscillating in a plane perpendicular to the $x - y$ plane of cell. On the other hand, 4th and 5th phonon bands represent the optical vibrations (out-of-phase) of Ta and Sb atoms in the $x - y$ plane of cell. These two optical phonon branches are degenerate along the $\Gamma - A$ path due to the crystal symmetry of TaSb compound. At a $q$-point below the TDP, the acoustic mode (3rd band) has lower frequency than that of the optical modes (4 and 5). However, above the TDP, the acoustic mode unusually attains higher frequency compared to the frequency of the optical modes, thus leading to a band-inversion in the phonon spectra along with formation of a triple-degenerate-point along $\Gamma - A$ path. Also, the Ta atom oscillates with a larger amplitude in the inverted acoustic mode (3rd band). The TDP is protected by the $C_{3v}$ rotational symmetry of the TaSb crystal. The excitations near the TDP yield three-component bosonic quasiparticles in the present system, which enormously suppress the lattice thermal conductivity.

The competition of the in-plane and out-of-plane interatomic force constants between the atoms of comparable mass could be the primary reason of the phonon-band inversion in TaSb and TaBi compounds. Therefore, we study the vibrational modes of a diatomic system considering a harmonic approximation for the interatomic potential. Our analysis suggests that the frequency gap ($\Delta$) between the optical (branch 4 or 5 ) and acoustic phonon branches (branch 3) at the BZ edge (0, 0, $\frac{\pi}{2}$) is:

$$\Delta = \sqrt{\frac{2\beta_{\parallel}}{m}} - \sqrt{\frac{2\beta_{\perp}}{M}} \tag{1}$$

*i.e.*,

$$\Delta \propto \sqrt{\beta_{\parallel}} - \sqrt{\beta_{\perp}\frac{m}{M}} \tag{2}$$

Here, $\beta_{\parallel}$ and $\beta_{\perp}$ are the in-plane and out-of-plane second-order interatomic force constants between the atoms of mass $m$ and $M$ ($m < M$), respectively. We observe that the frequency gap ($\Delta$) decreases systematically with increase in the $m/M$ ratio. For TaN ($m/M$ = 0.0774), TaP ($m/M$ = 0.1711), and TaAs ($m/M$ = 0.414) compounds $\Delta$ the obtained $\Delta$ is 200.5, 115.1, and 14.4 cm$^{-1}$, respectively. Interestingly, for TaSb ($m/M$ = 0.6731) and TaBi ($m/M$ = 0.8658) compounds $\Delta$ becomes negative (-16.7 and -27.8 cm$^{-1}$ respectively) indicating an abnormal inversion of phonon bands near the BZ edge (see SI for details). In addition to increasing $m/M$ ratio, $\beta_{\perp} > \beta_{\parallel}$ condition is essential to observe the phonon band-inversion at the BZ edge.

In order to further test the validity of Eq. 2 for phonon band-inversion, we apply it on the data reported by Li et al. [32]. Figure 6 shows the calculated $\Delta$ ($= \sqrt{\beta_{\parallel}} - \sqrt{\beta_{\perp}\frac{m}{M}}$) for nine different compounds using the data from Ref. [32]. Here, we used normalized $\Delta$ by dividing it by the constant factors. Used atomic masses are given in Table I. We notice that only three out of nine compounds can have negative $\Delta$, and therefore only these three compounds (TiS, ZrSe, and HfTe) can host TDP in their phonon spectrum, which is consistent with the predictions in Ref. [32].

### A. Phonons surface states in TaSb

The non-trivial topology of phonons bandstructure in a system implies the possibility of hosting topologically protected gapless surface states. Therefore, in order to confirm the non-trivial nature of phonon spectra and the

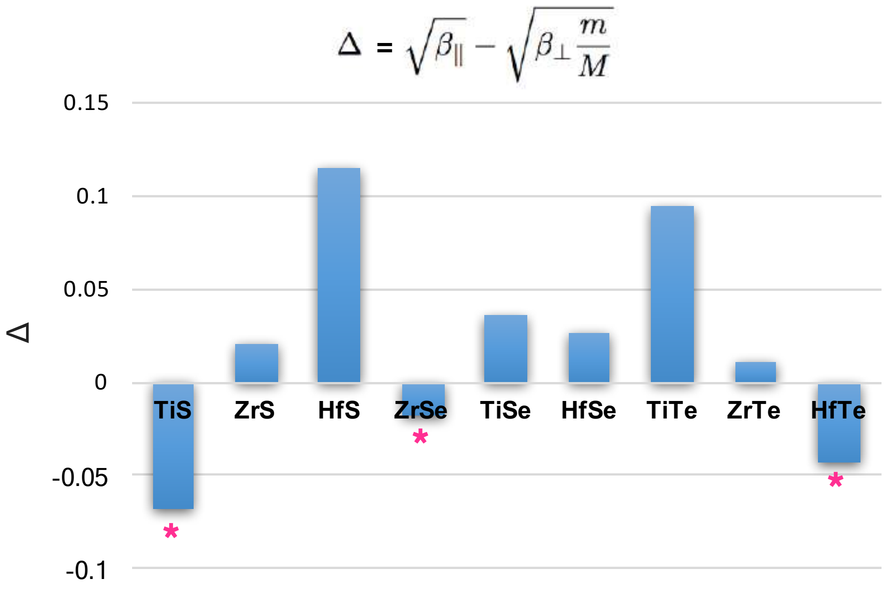


FIG. 6: (Color online) Normalized phonon frequency gap (Δ) calculated near the A-point of BZ for the set of nine compounds reported in Ref. [32]. A negative value of Δ implies the presence of phonon band-inversion. Only three compounds (marked with asterisk) show negative Δ.

existence of gapless surface states, we calculate the surface state spectrum of phonons using the method described in the SI. Fig. 7 shows the (001) and (100) surface phonon spectra for TaSb compound. We observe gapless phonon surface states at the Γ point for both surfaces. Since there is no bulk frequency gap in the phonon spectra of TaSb, the surface phonon bands are buried within the bulk bands. Hence, it could be experimentally challenging to detect the gapless phonon surface states in TaSb compound.

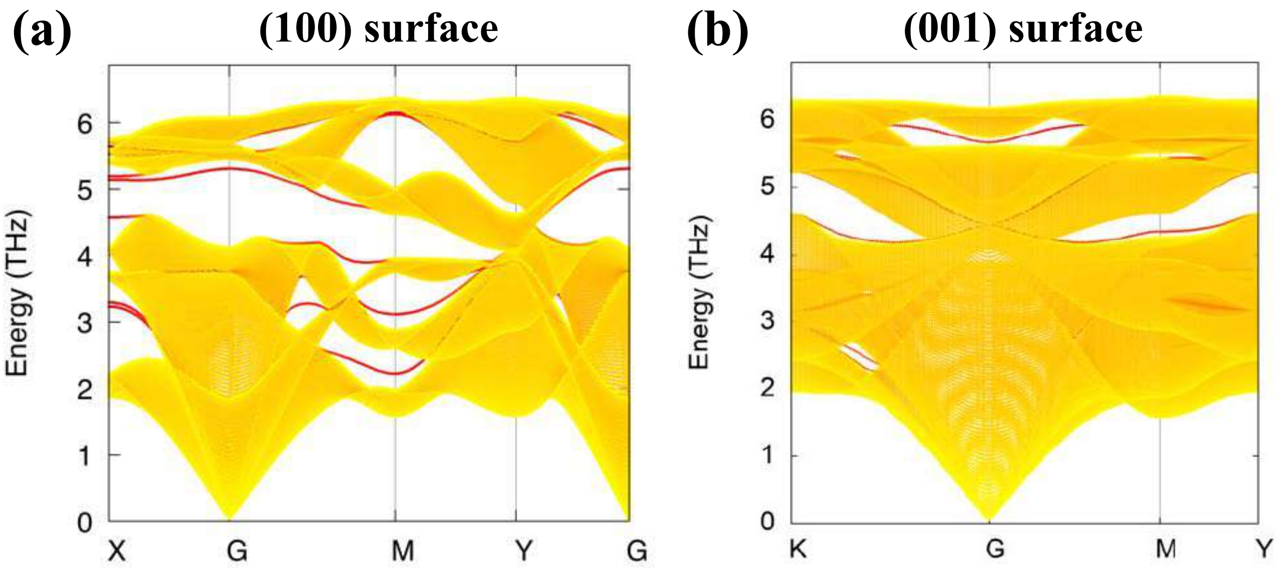


FIG. 7: (Color online) The phonon bandstructure calculated (a) at (100) surface and (b) at (001) TaSb surface. The red lines represents the surface bands while the yellow lines represent the bulk bands.

### B. Theoretical demonstration of the non-trivial topology of phonon modes in TaSb

Assuming $u^{\alpha}_{l,s}$ is the displacement of the $s^{th}$ atom in the $l^{th}$ unit cell along $\alpha$ ($\alpha = x, y, z$) direction, the total potential can be expanded according to $u^{\alpha}_{l}$ as

$$\Phi = \Phi_0 + \frac{1}{2}\sum_{l,s,\alpha}\sum_{l',s',\beta}\Phi^{l-l'}_{\alpha\beta,ss'}u^{\alpha}_{l,s}u^{\beta}_{l',s'} + ... \tag{3}$$

where the first derivation is zero due to the equilibrium state. The second derivation coefficient represents the force constant which can be calculated in the first-principle calculations. There is a very important relation

$$\sum_{l'}\Phi^{l-l'}_{\alpha\beta,ss'} = 0 \tag{4}$$

So $\Phi^{0}_{\alpha\beta,ss'} = -\sum_{l\neq 0}\Phi^{l}_{\alpha\beta,ss'}$

In TaSb system, $s$=Ta, $s'$=Sb. Under the $C_{3v}$ symmetry, $\Phi^{0}_{xx,ss}$ should be the same as $\Phi^{0}_{yy,ss}$, which leads to a trivial nodal line linking two triple points along $A-\Gamma-A$ shown in Fig. 8(a) and Fig. 8(e). A trivial nodal line means that the Berry phase along a close around the nodal line, like $S^1$ in Fig. 8(e), is zero. In order to study the topological structure of the nodal line in the spinless system, we studied two cases by manually modifying the lattice constant. One is that $\Phi^{0}_{xx,Ta-Ta} \neq \Phi^{0}_{yy,Ta-Ta}$, the other is $\Phi^{0}_{xx,Sb-Sb} \neq \Phi^{0}_{yy,Sb-Sb}$. The band structure and the nodal lines are shown in Fig. 8 (b-c) and Fig. 8 (f-g) respectively. It is shown that the trivial nodal line would deform to a non-trivial nodal line with $\pi$ Berry phase.

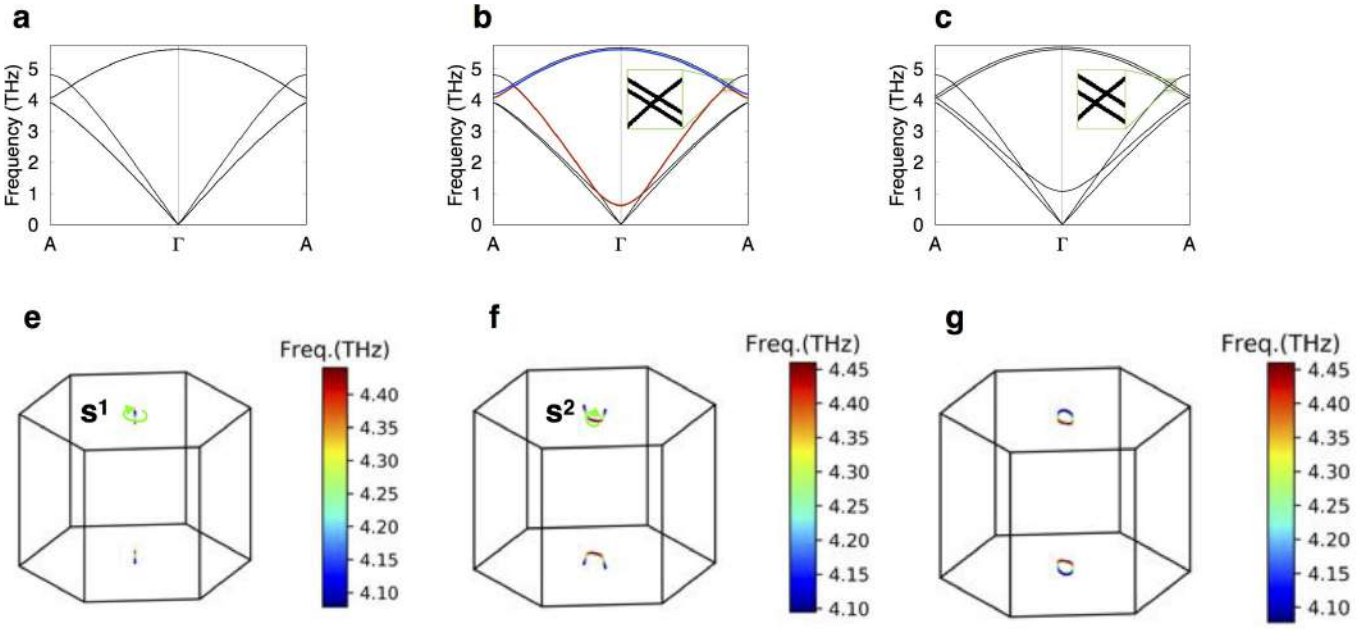


FIG. 8: Evolution of phonon band structure and nodal line with different tight binding models for TaSb. The nodal line represents touching points between the $3^{rd}$ band and the $4^{th}$ band indicated as red and blue lines in panel b respectively. More details are given in the main draft.

## V. ELECTRONIC BANDSTRUCTURE OF OTHER TRIPLE-POINT-METALS

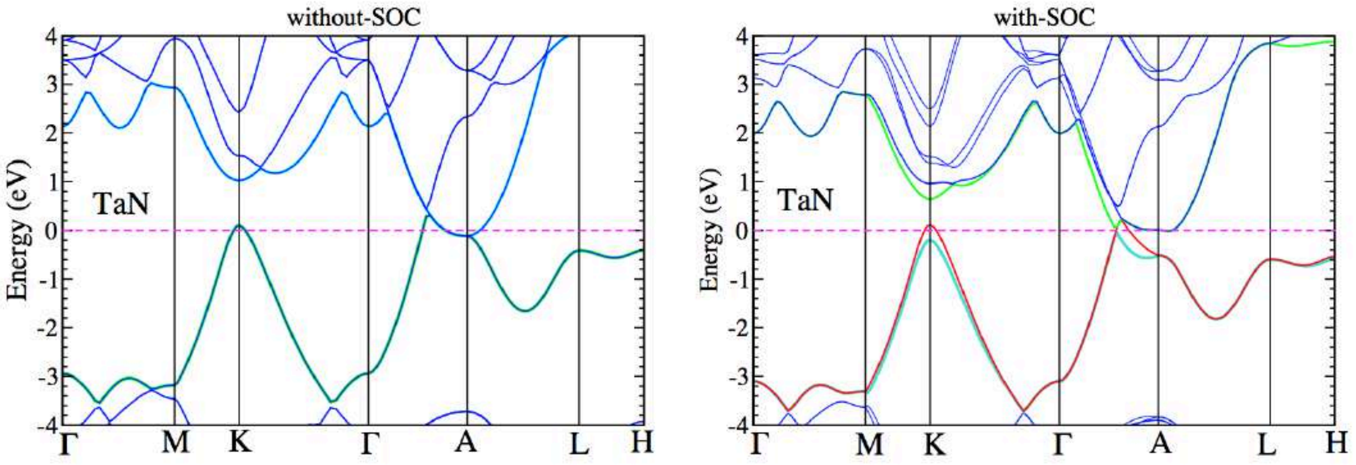


FIG. 9: Electronic bandstructure of TaN calculated without-SOC (left) and with-SOC (right).

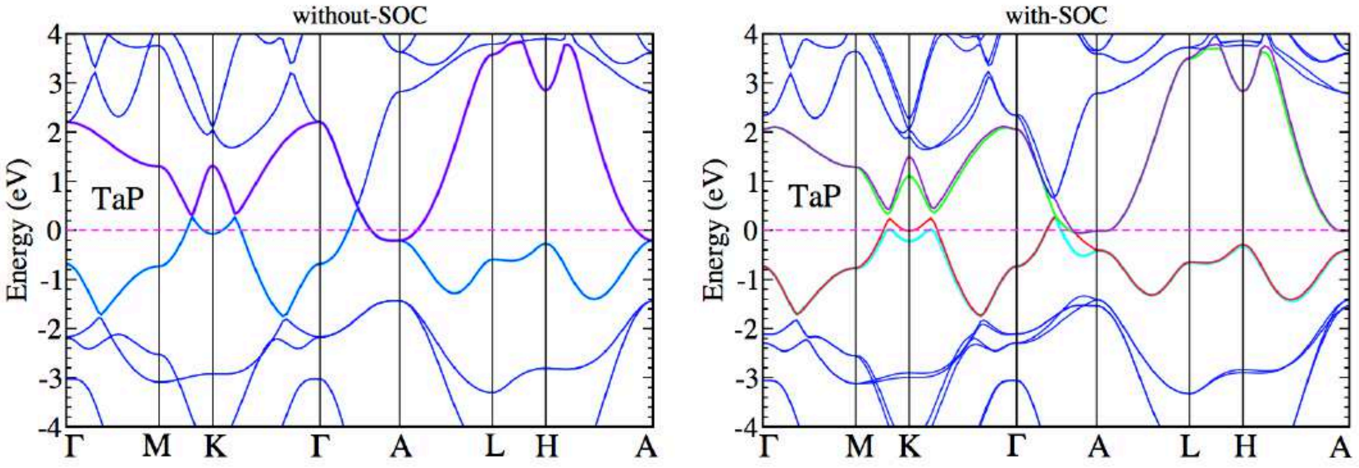


FIG. 10: Electronic bandstructure of TaP calculated without-SOC (left) and with-SOC (right).

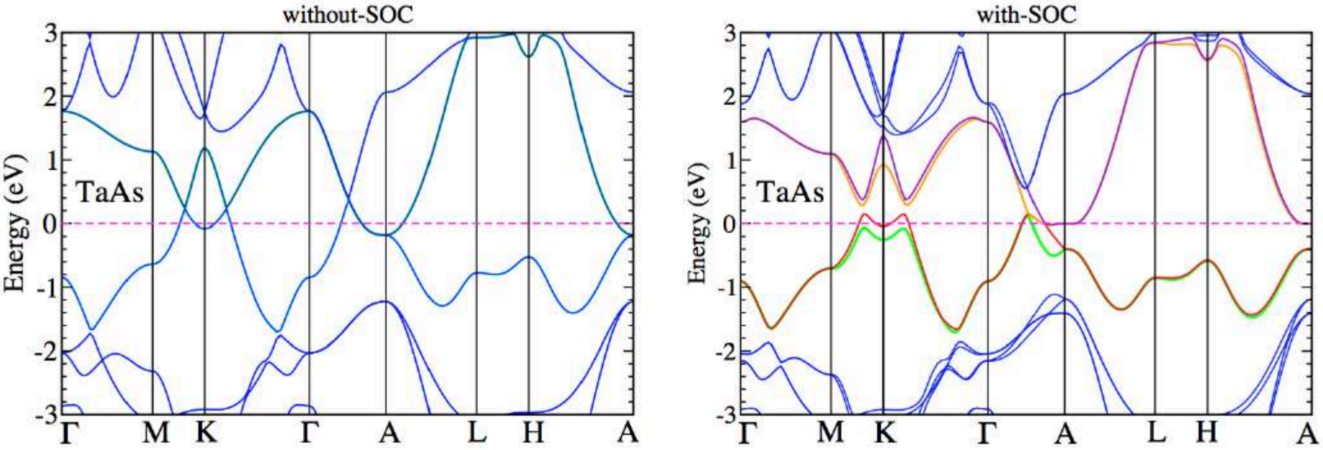


FIG. 11: Electronic bandstructure of TaAs calculated without-SOC (left) and with-SOC (right).

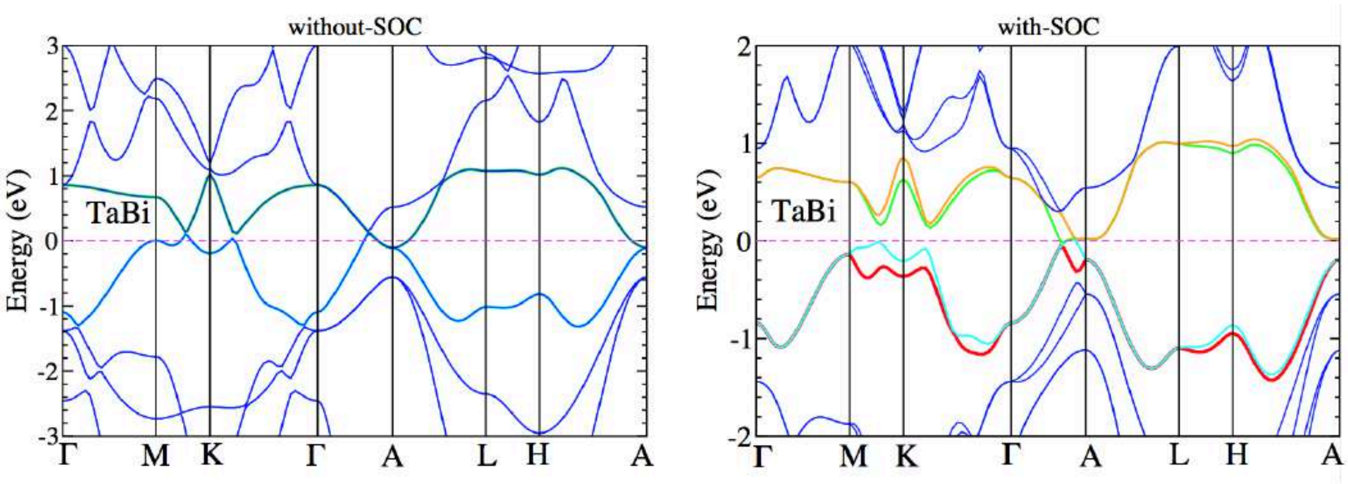


FIG. 12: Electronic bandstructure of TaBi calculated without-SOC (left) and with-SOC (right).

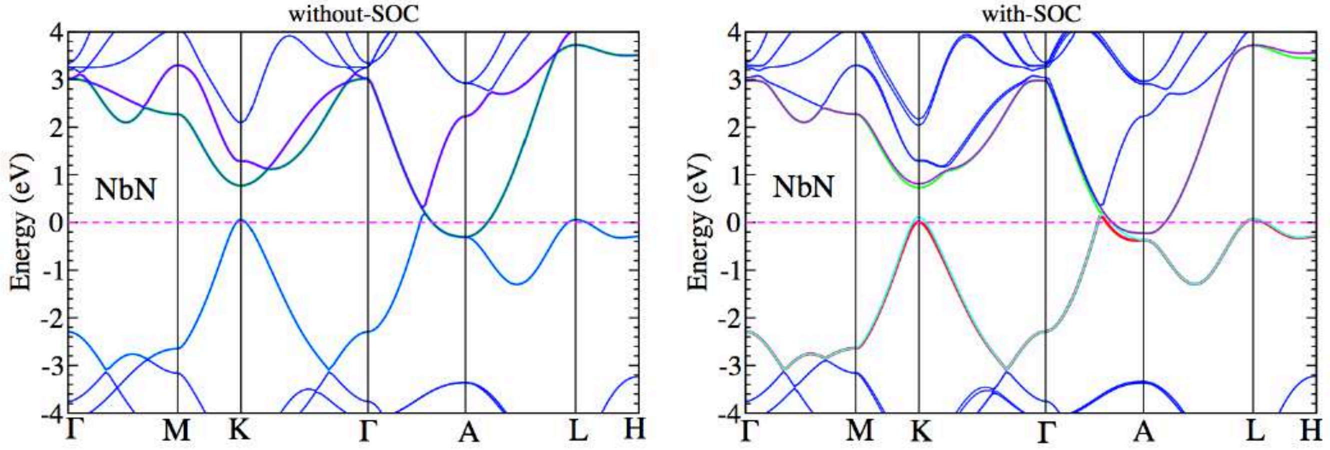


FIG. 13: Electronic bandstructure of NbN calculated without-SOC (left) and with-SOC (right).

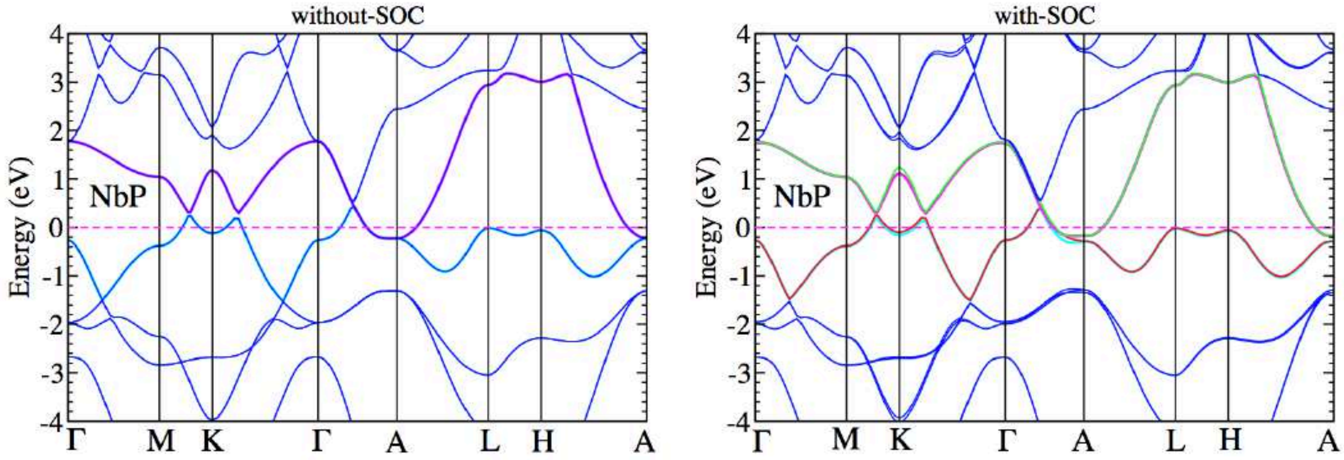


FIG. 14: Electronic bandstructure of NbP calculated without-SOC (left) and with-SOC (right).

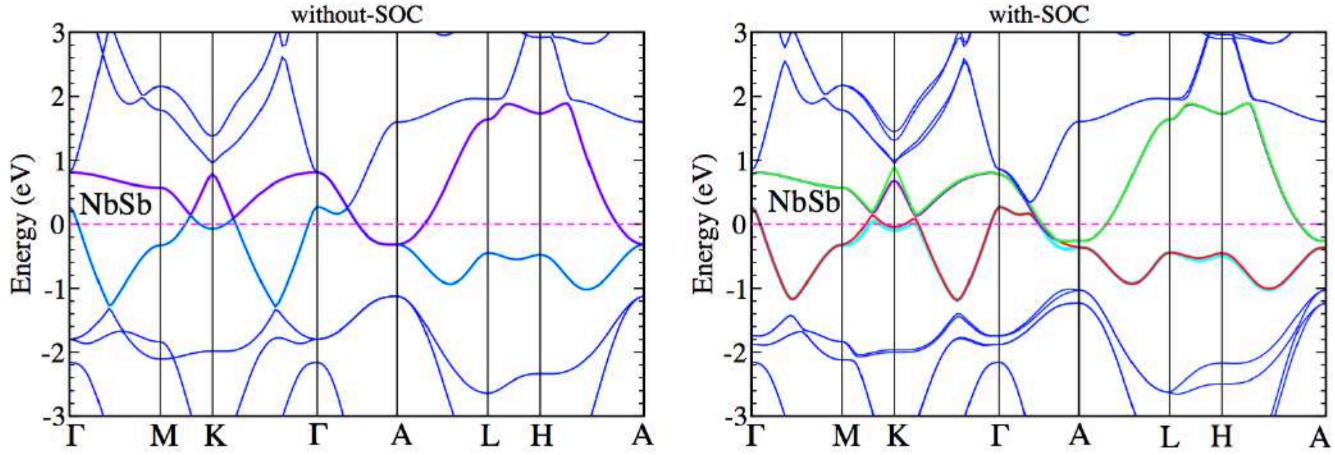


FIG. 15: Electronic bandstructure of NbSb calculated without-SOC (left) and with-SOC (right).

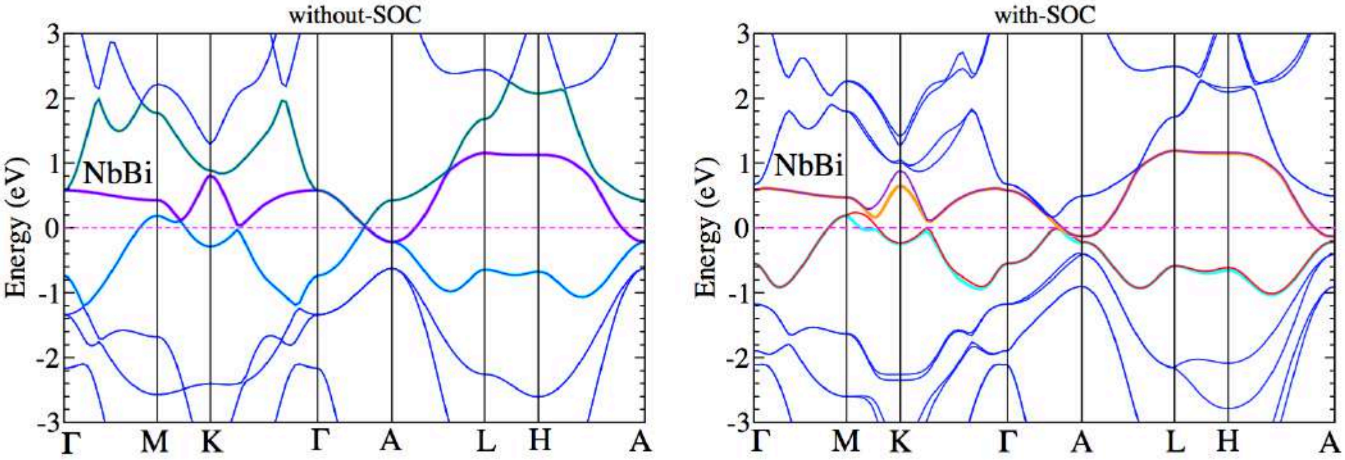


FIG. 16: Electronic bandstructure of NbBi calculated without-SOC (left) and with-SOC (right).

## VI. PHONON BANDSTRUCTURE OF OTHER TRIPLE-POINT-METALS

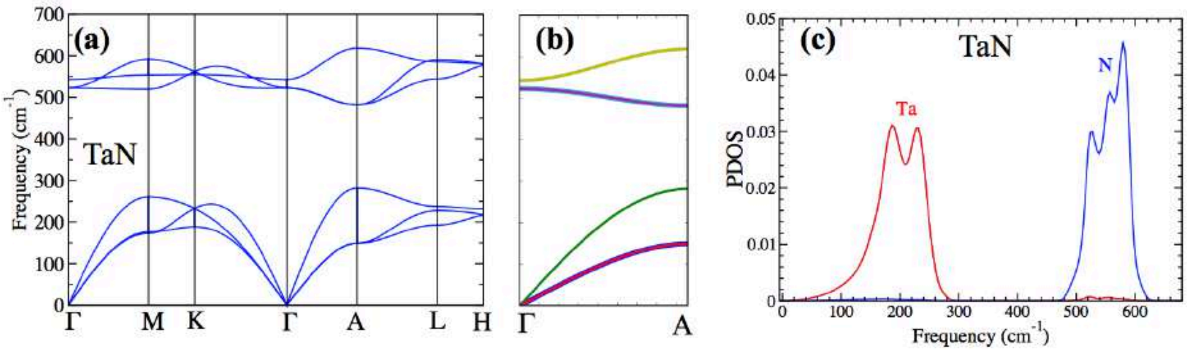


FIG. 17: (a) Calculated phonon bandstructure of TaN calculated along the high-symmetry directions in momentum space. (b) The phonon bandstructure calculated along the Γ–A path. The color of bands represent the phonon eigen modes. (c) Atom projected partial phonon density of states (PDOS). Red and blue colors depict the PDOS for Ta and N atoms, respectively.

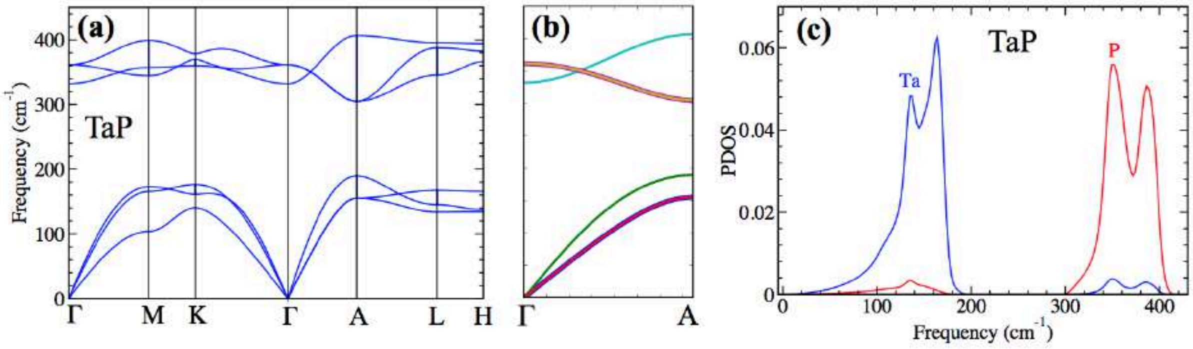


FIG. 18: (a) Calculated phonon bandstructure of TaP calculated along the high-symmetry directions in momentum space. (b) The phonon bandstructure calculated along the Γ–A path. The color of bands represent the phonon eigen modes. (c) Atom projected partial phonon density of states (PDOS). Red and blue colors depict the PDOS for Ta and P atoms, respectively.

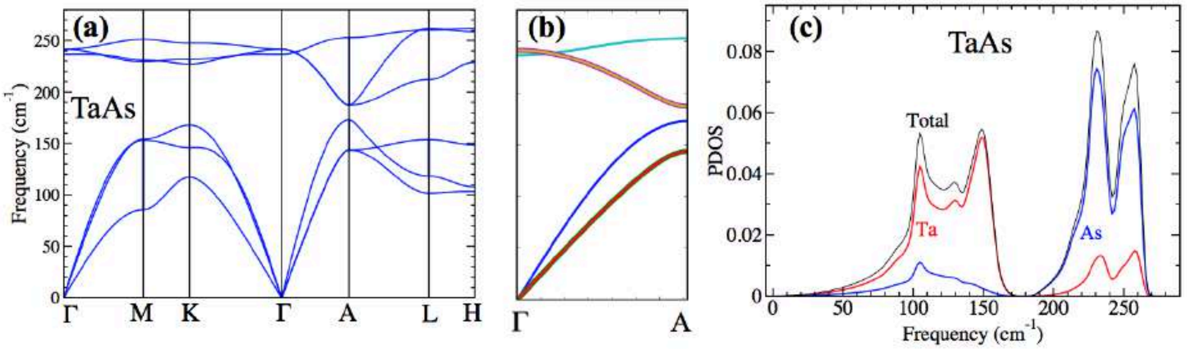


FIG. 19: (a) Calculated phonon bandstructure of TaAs calculated along the high-symmetry directions in momentum space. (b) The phonon bandstructure calculated along the Γ–A path. The color of bands represent the phonon eigen modes. (c) Atom projected partial phonon density of states (PDOS). Red and blue colors depict the PDOS for Ta and As atoms, respectively.

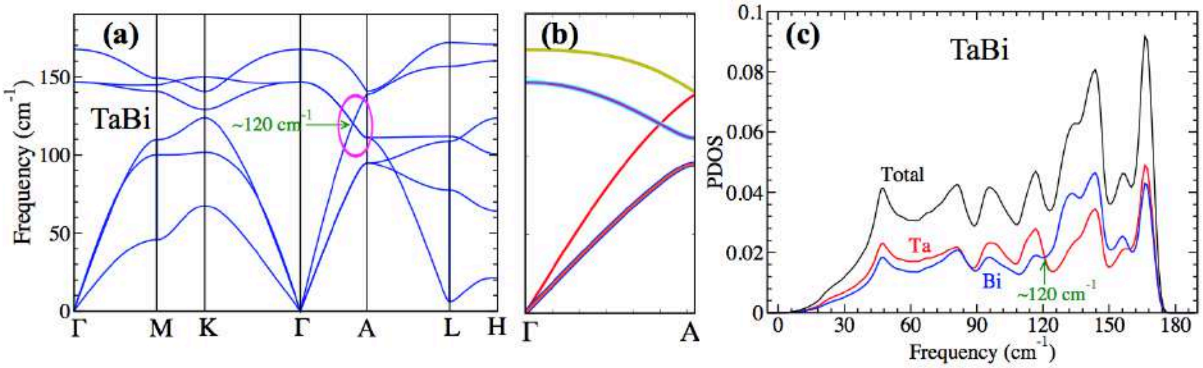


FIG. 20: (a) Calculated phonon bandstructure of TaBi calculated along the high-symmetry directions in momentum space. (b) The phonon bandstructure calculated along the Γ–A path. The color of bands represent the phonon eigen modes. (c) Atom projected partial phonon density of states (PDOS). Red and blue colors depict the PDOS for Ta and Bi atoms, respectively.

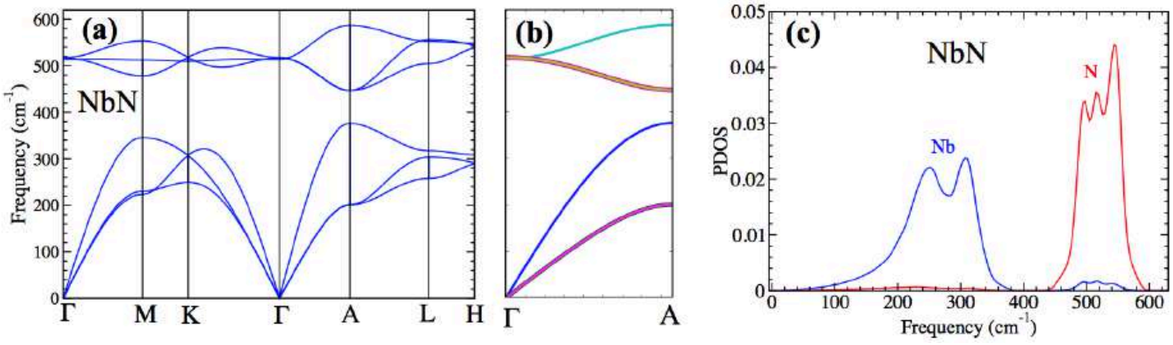


FIG. 21: (a) Calculated phonon bandstructure of NbN calculated along the high-symmetry directions in momentum space. (b) The phonon bandstructure calculated along the Γ–A path. The color of bands represent the phonon eigen modes. (c) Atom projected partial phonon density of states (PDOS). Red and blue colors depict the PDOS for Nb and N atoms, respectively.

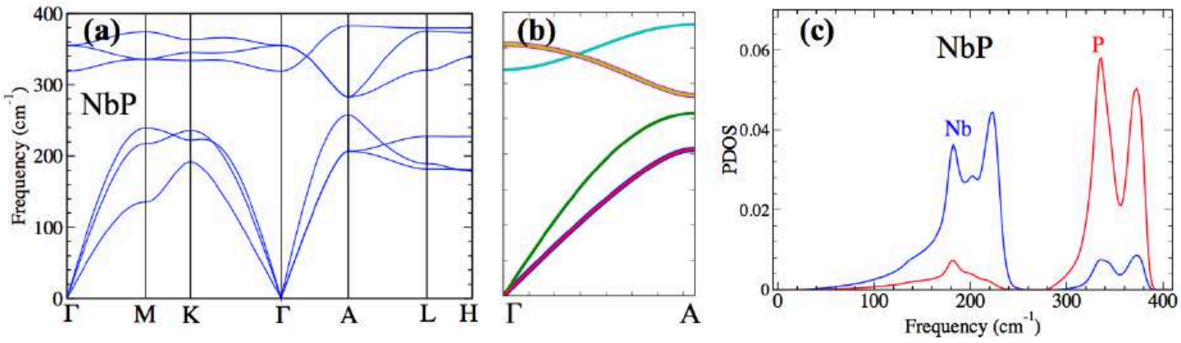


FIG. 22: (a) Calculated phonon bandstructure of NbP calculated along the high-symmetry directions in momentum space. (b) The phonon bandstructure calculated along the Γ–A path. The color of bands represent the phonon eigen modes. (c) Atom projected partial phonon density of states (PDOS). Red and blue colors depict the PDOS for Nb and P atoms, respectively.

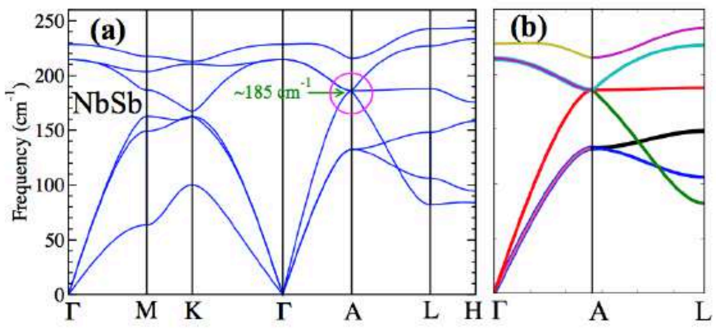


FIG. 23: (a) Calculated phonon bandstructure of NbSb calculated along the high-symmetry directions in momentum space. (b) The phonon bandstructure calculated along the Γ–A path. The color of bands represent the phonon eigen modes. (c) Atom projected partial phonon density of states (PDOS). Red and blue colors depict the PDOS for Nb and Sb atoms, respectively.

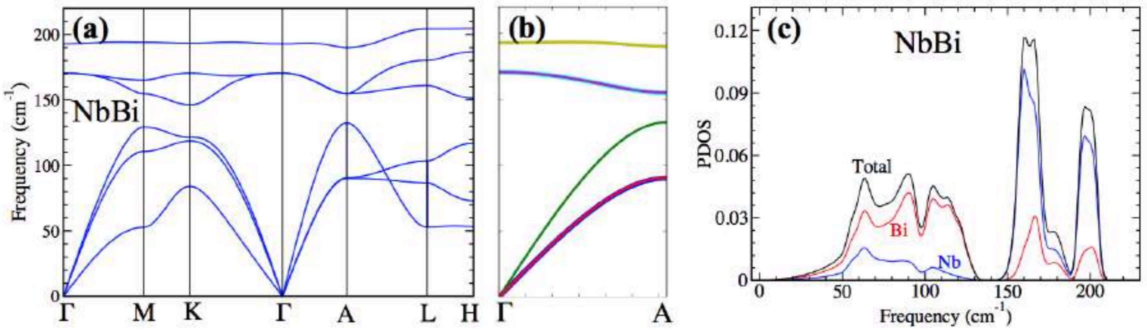


FIG. 24: (a) Calculated phonon bandstructure of NbBi calculated along the high-symmetry directions in momentum space. (b) The phonon bandstructure calculated along the Γ–A path. The color of bands represent the phonon eigen modes. (c) Atom projected partial phonon density of states (PDOS). Red and blue colors depict the PDOS for Nb and Bi atoms, respectively.

## VII. COMPARISON OF PHONON MEAN FREE PATH IN TaSb AND TaN

In order to understand the role of TDP on the phonon mean free path, we compare the calculated phonon mean free path in TaSb and TaN, both having iso-structure and iso-electronic properties. TaSb hosts TDP whereas TaN lacks TDP in the phonon spectrum. We find the phonon mean free path decreases by almost two-orders in magnitude due to the enhanced phonon-scattering by TDP in TaSb [Fig. 25]. This is the main reason behind reduction in the lattice thermal conductivity in the compounds hosting TDP.

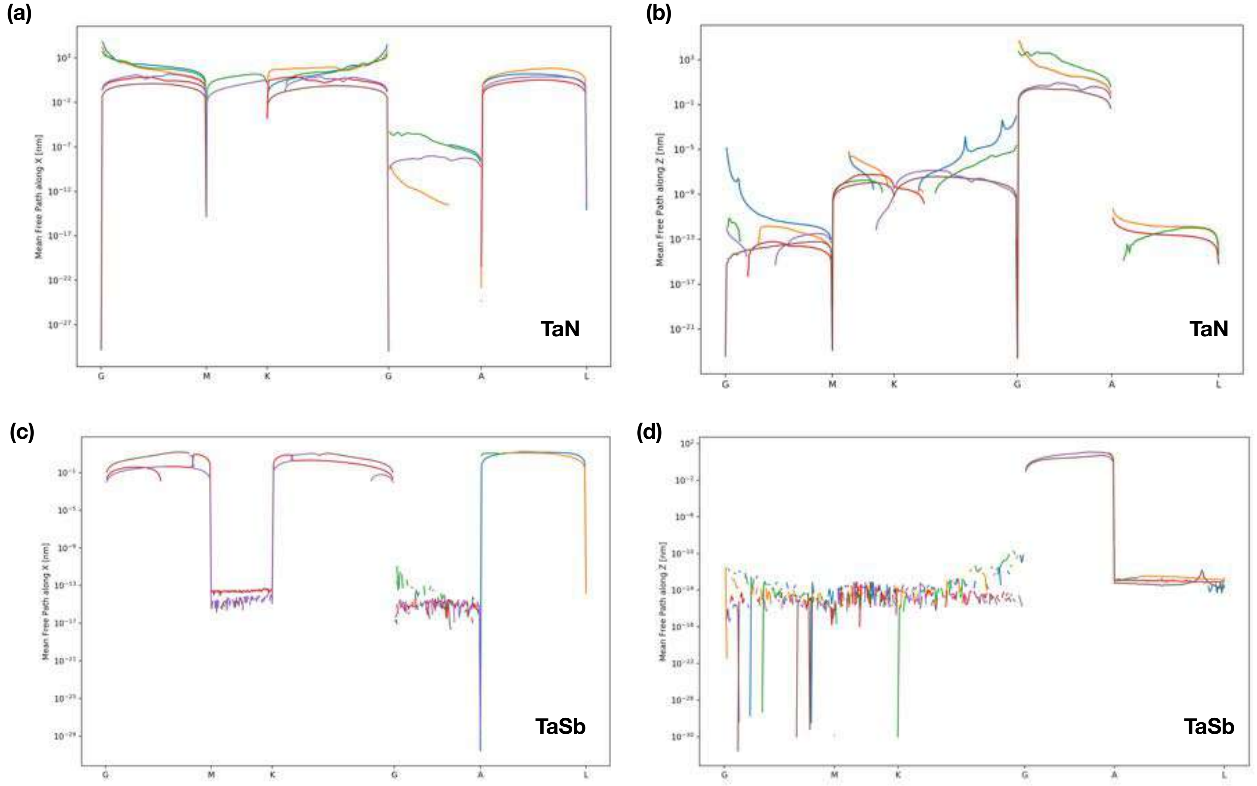


FIG. 25: (a) Calculated phonon mean free for TaN (a-b) and for TaSb (c-d).

## VIII. THERMAL CONDUCTIVITY

Here we compare the thermal conductivity $\kappa_{total}$, and its different contributions - electronic ($\kappa_{el}$ ) and lattice ($\kappa_{ph}$), of TaSb and TaBi with TaN and TaP (compounds that do not host TDP in their phonon spectra). At low temperatures (T), the $\kappa_{ph}$ term dominates the total thermal conductivity, whereas $\kappa_{el}$ term takes over at high T

due to the metallicity in TaX. In Fig. 26 one can notice that the $\kappa_{ph}$ decreases considerably (almost two orders in magnitude) in TaSb and TaBi compared to that of in TaN and TaP. This can attributed to the reduced phonon mean path in TaSb and TaBi due to the presence of TDP in their phonon spectra. $\kappa_{ph}$ is lower in-plane $(x-y)$ since two in-plane optical phonon modes scatter one out-of-plane acoustic phonon mode, causing larger reduction in $\kappa_{ph}$ in the $x-y$ plane. On the other hand, $\kappa_{el}$ is almost in the same order of magnitude for all TaX compounds at low temperature and low doping concentrations. Nonetheless, $\kappa_{total}$ is smaller in TaSb and TaBi compared to the TaN and TaP at low temperature and low doping concentrations.

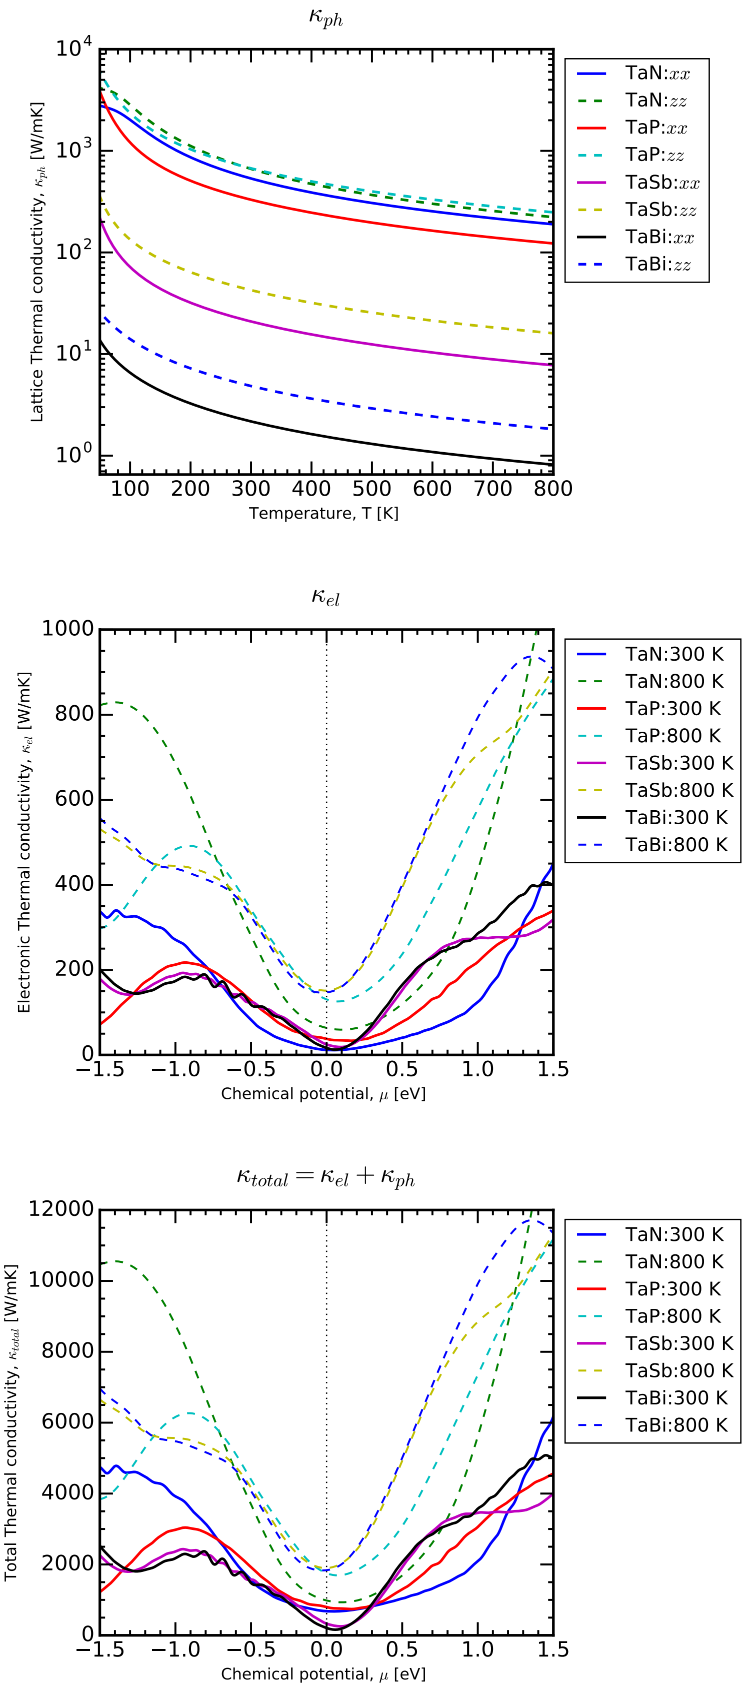


FIG. 26: Comparison of different components of lattice thermal conductivity, electronic thermal conductivity and total thermal conductivity along different directions in crystal at different temperatures. The $xx$ and $yy$ components of thermal conductivity tensor are same due to the crystal symmetry.

## IX. COMPARISON OF ELECTRONIC DENSITY OF STATES (DOS)

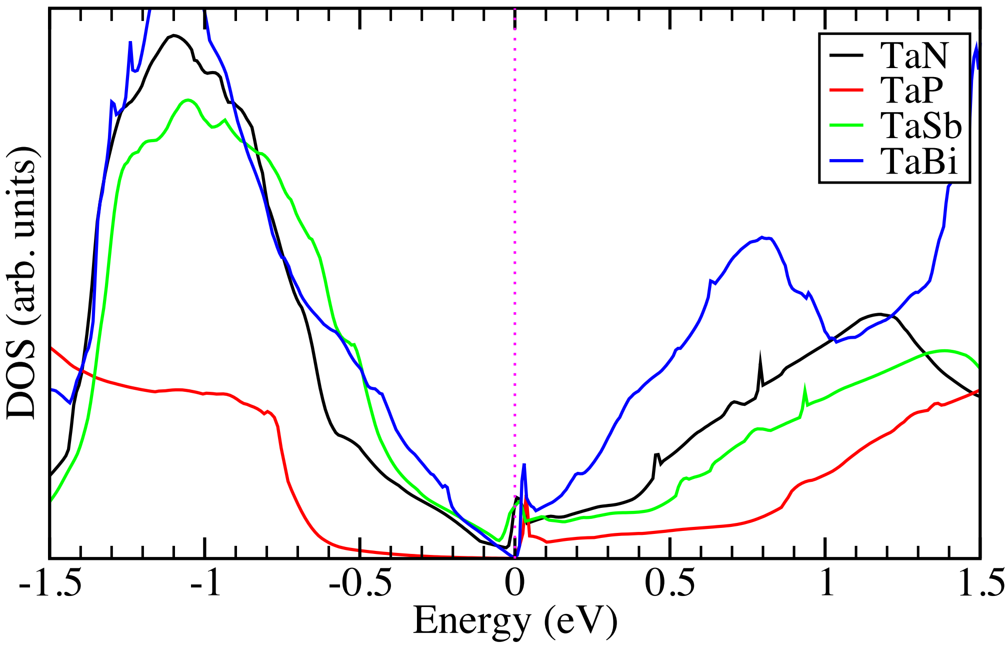


FIG. 27: Comparison of electronic density of states (DOS) in TaN, TaP, TaSb and TaBi. The dotted magenta line represents Fermi-level.

## X. THERMOELECTRIC PROPERTIES

Now we present the plots associated with the thermoelectric properties of TaX, as well for two compounds TiS and HfTe that are predicted to host TDP in their phonon spectra [32].

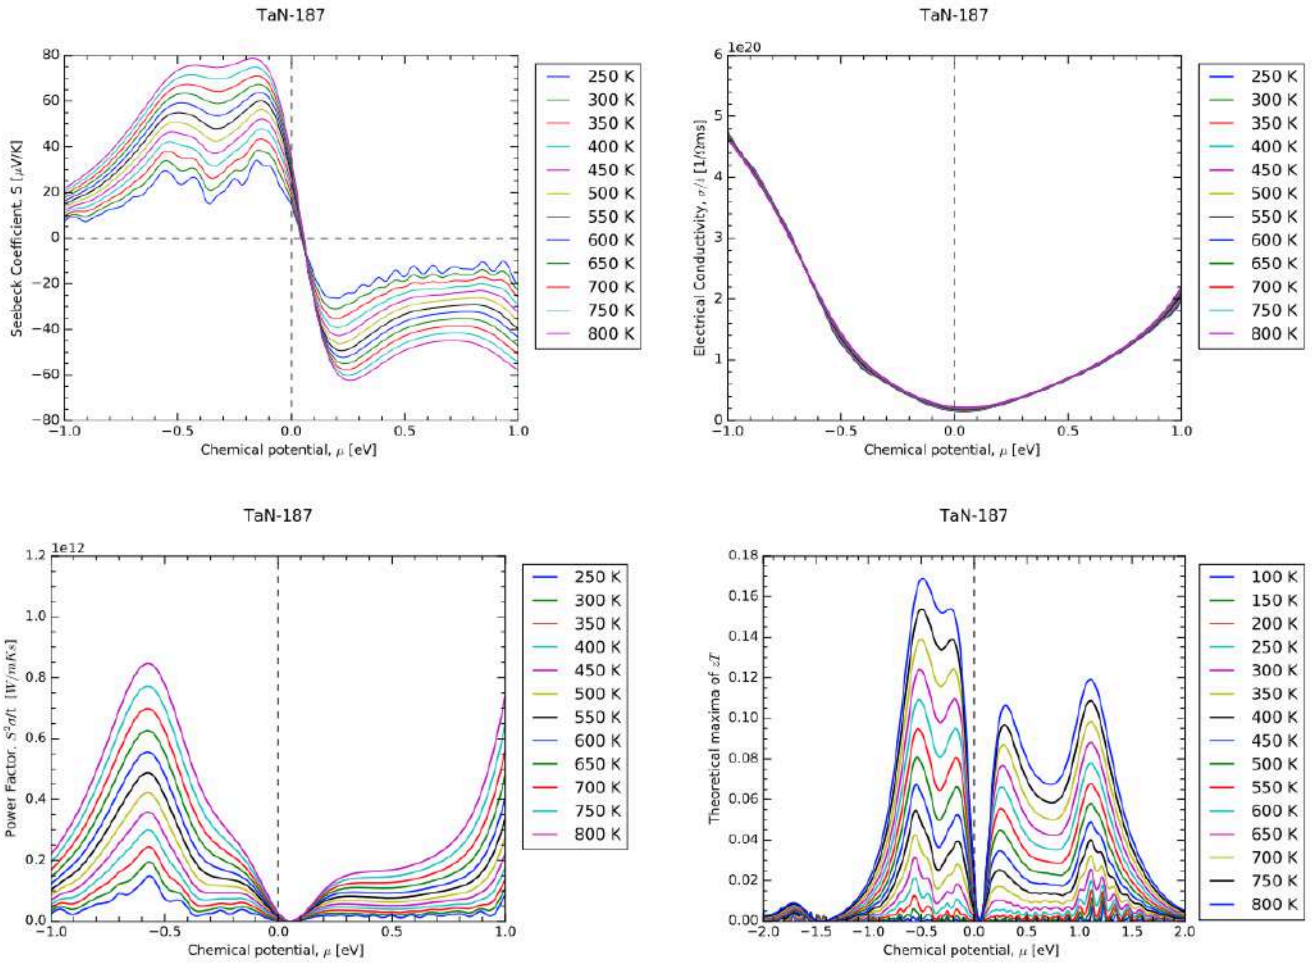


FIG. 28: Thermoelectric properties of TaN calculated using BoltzTrap code.

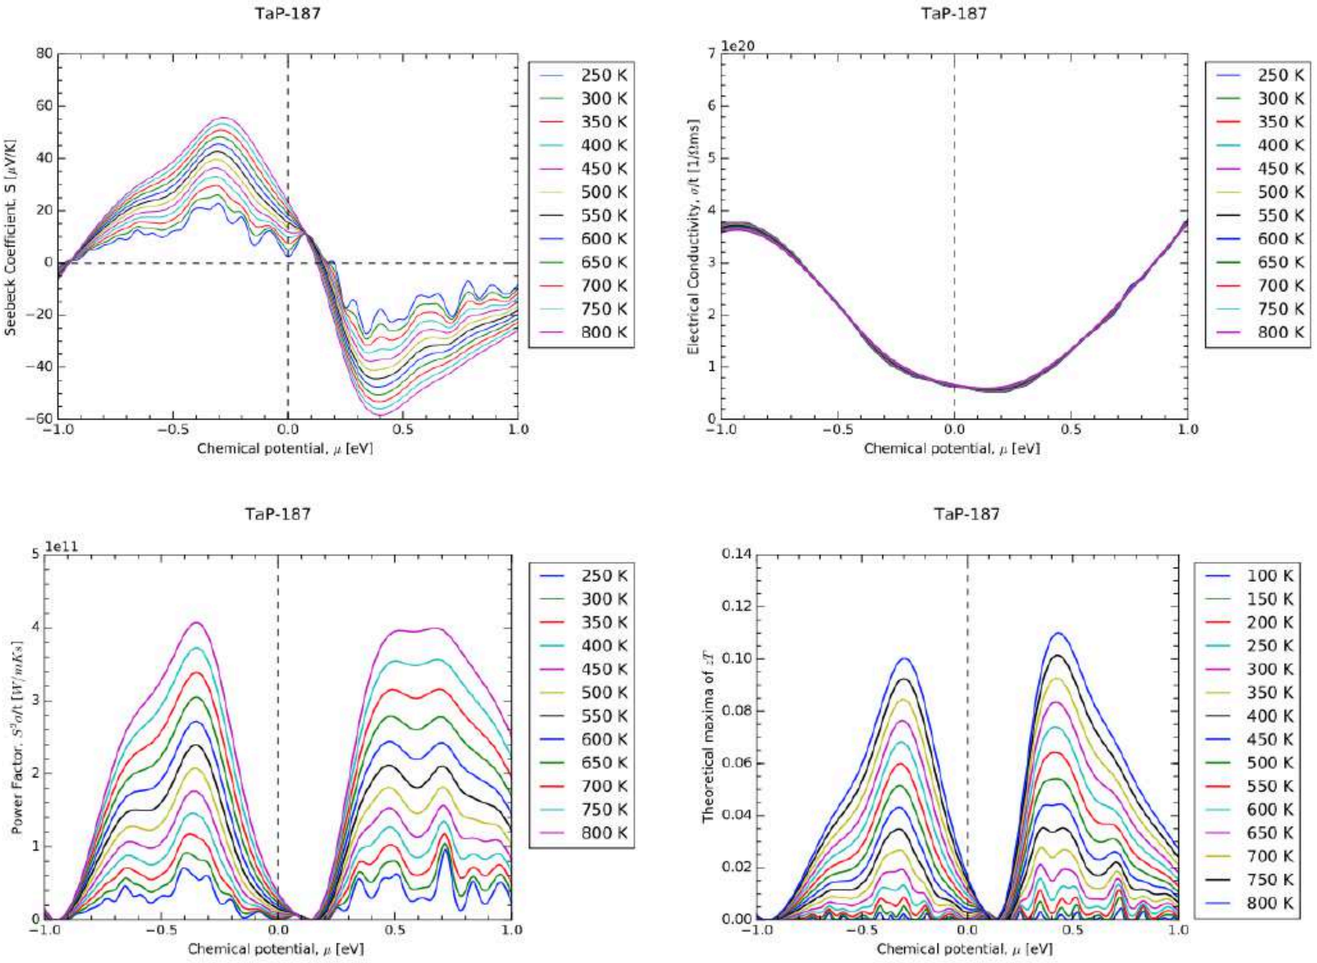


FIG. 29: Thermoelectric properties of TaP calculated using BoltzTrap code.

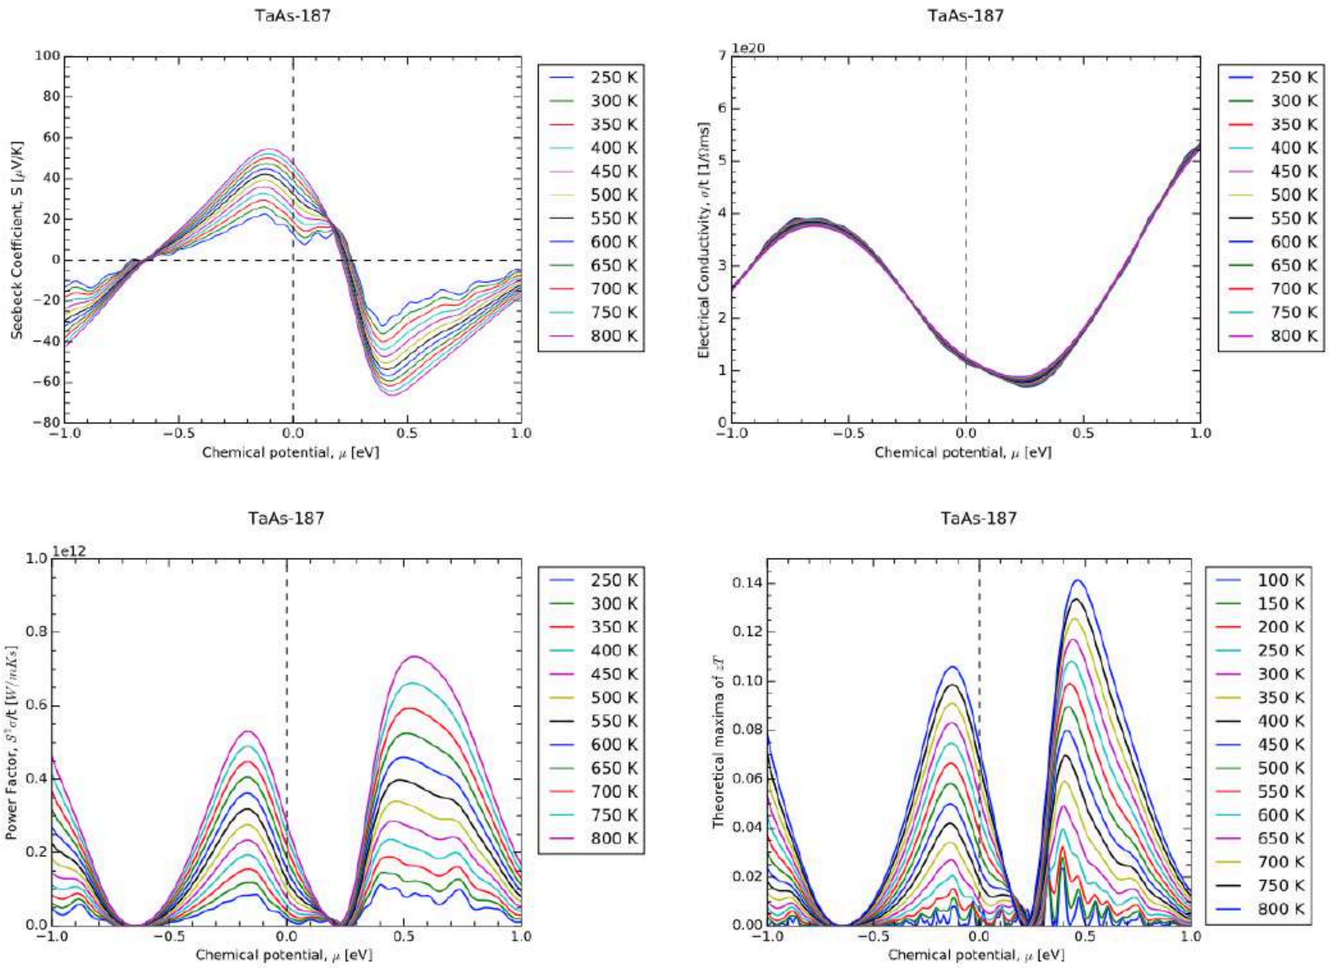


FIG. 30: Thermoelectric properties of TaAs calculated using BoltzTrap code.

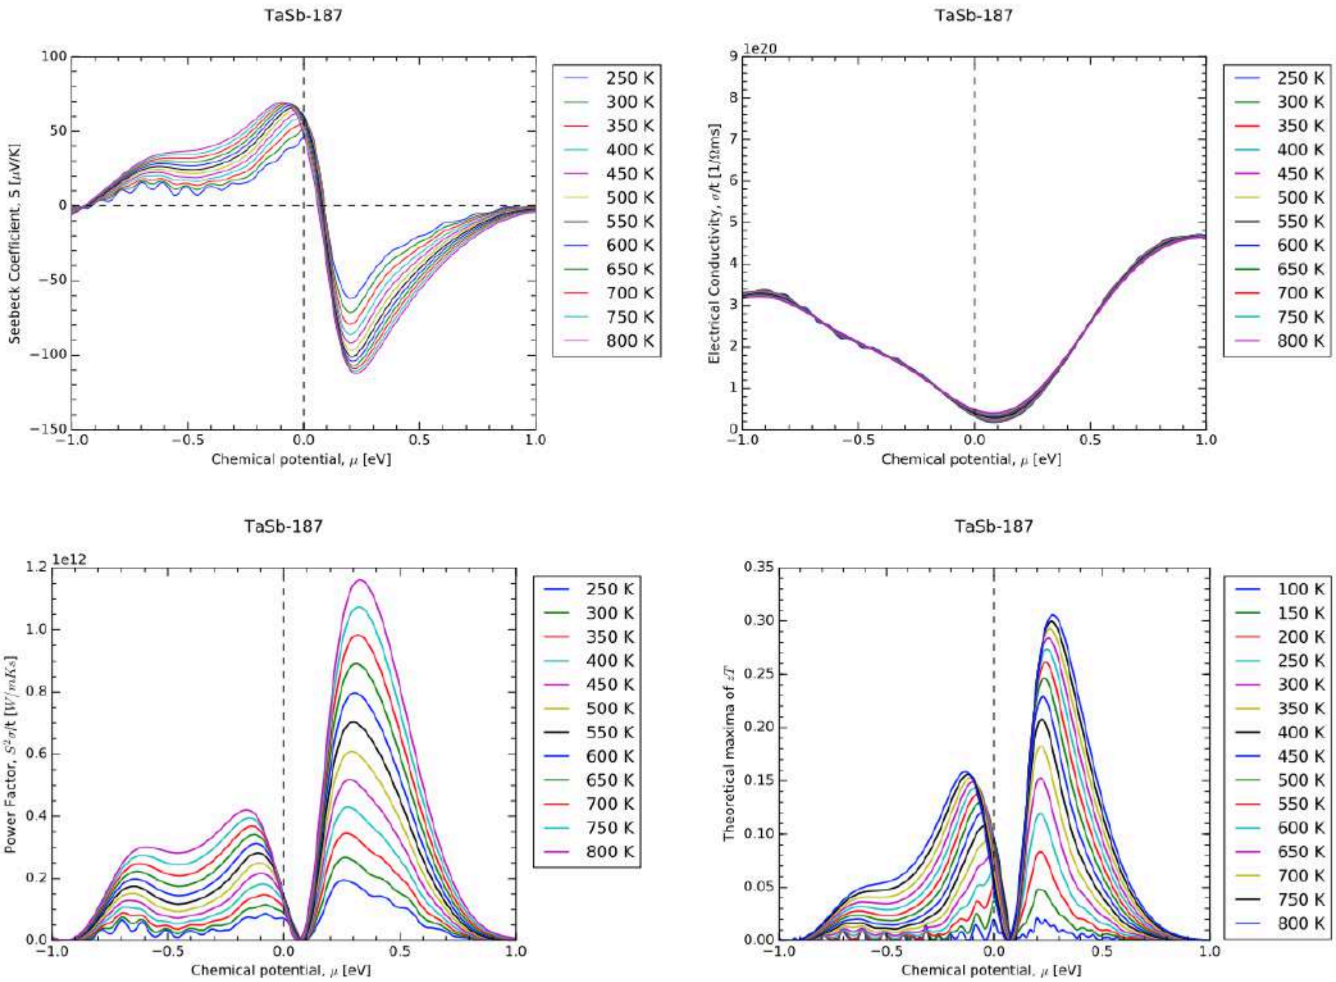


FIG. 31: Thermoelectric properties of TaSb calculated using BoltzTrap code.

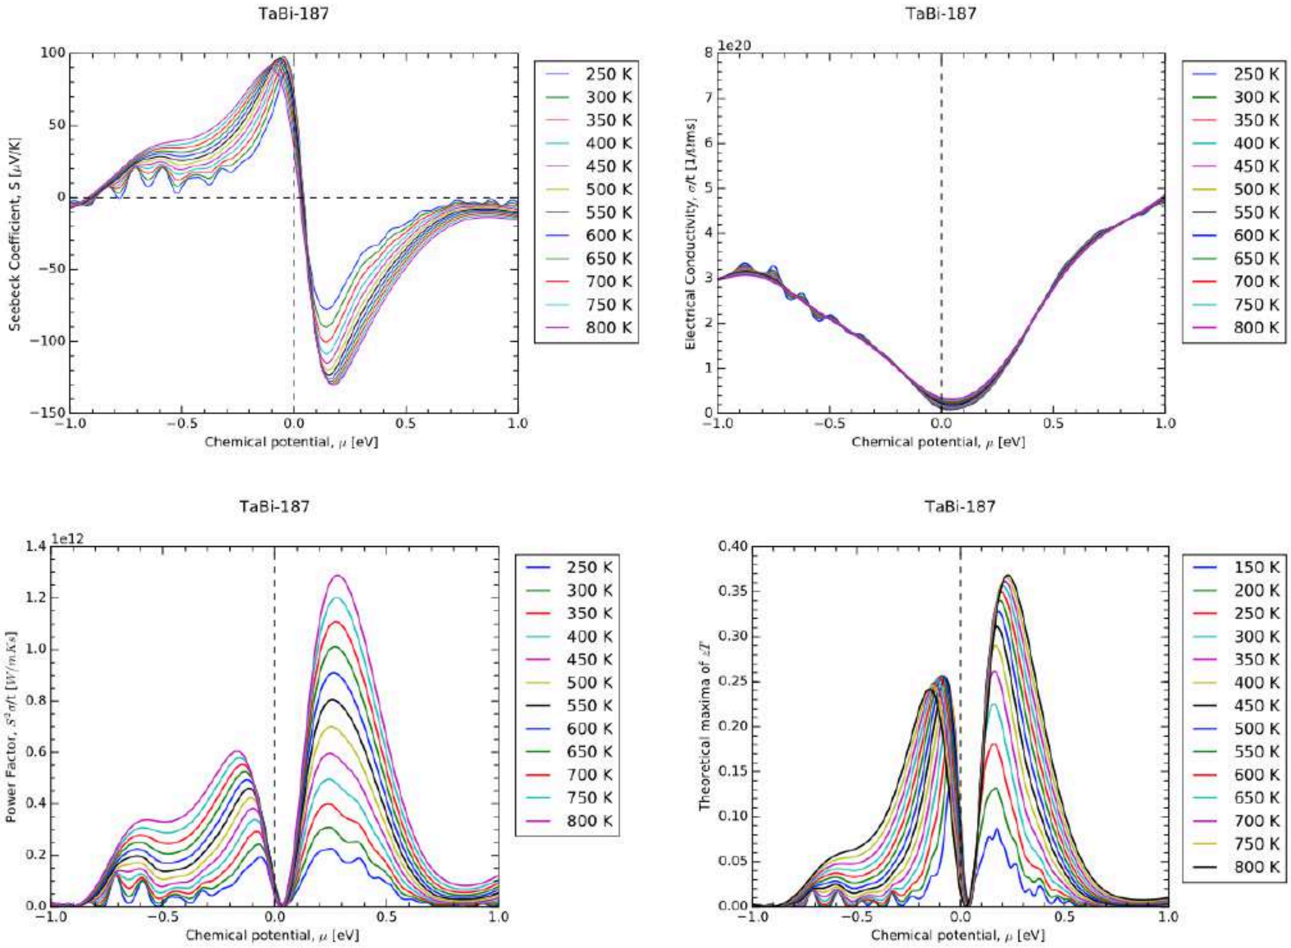


FIG. 32: Thermoelectric properties of TaBi calculated using BoltzTrap code.

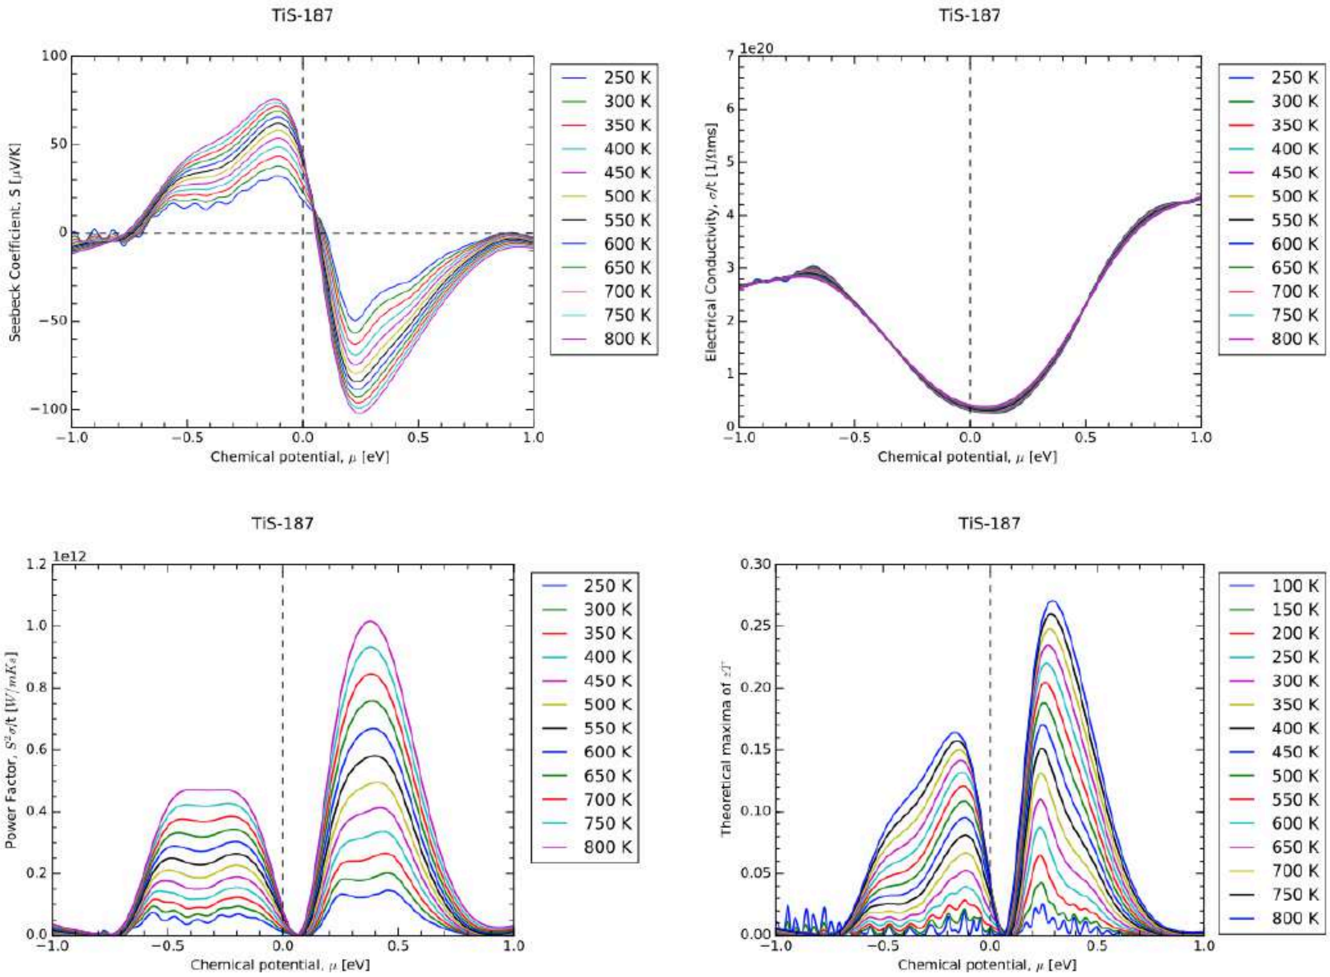


FIG. 33: Thermoelectric properties of TiS calculated using BoltzTrap code.

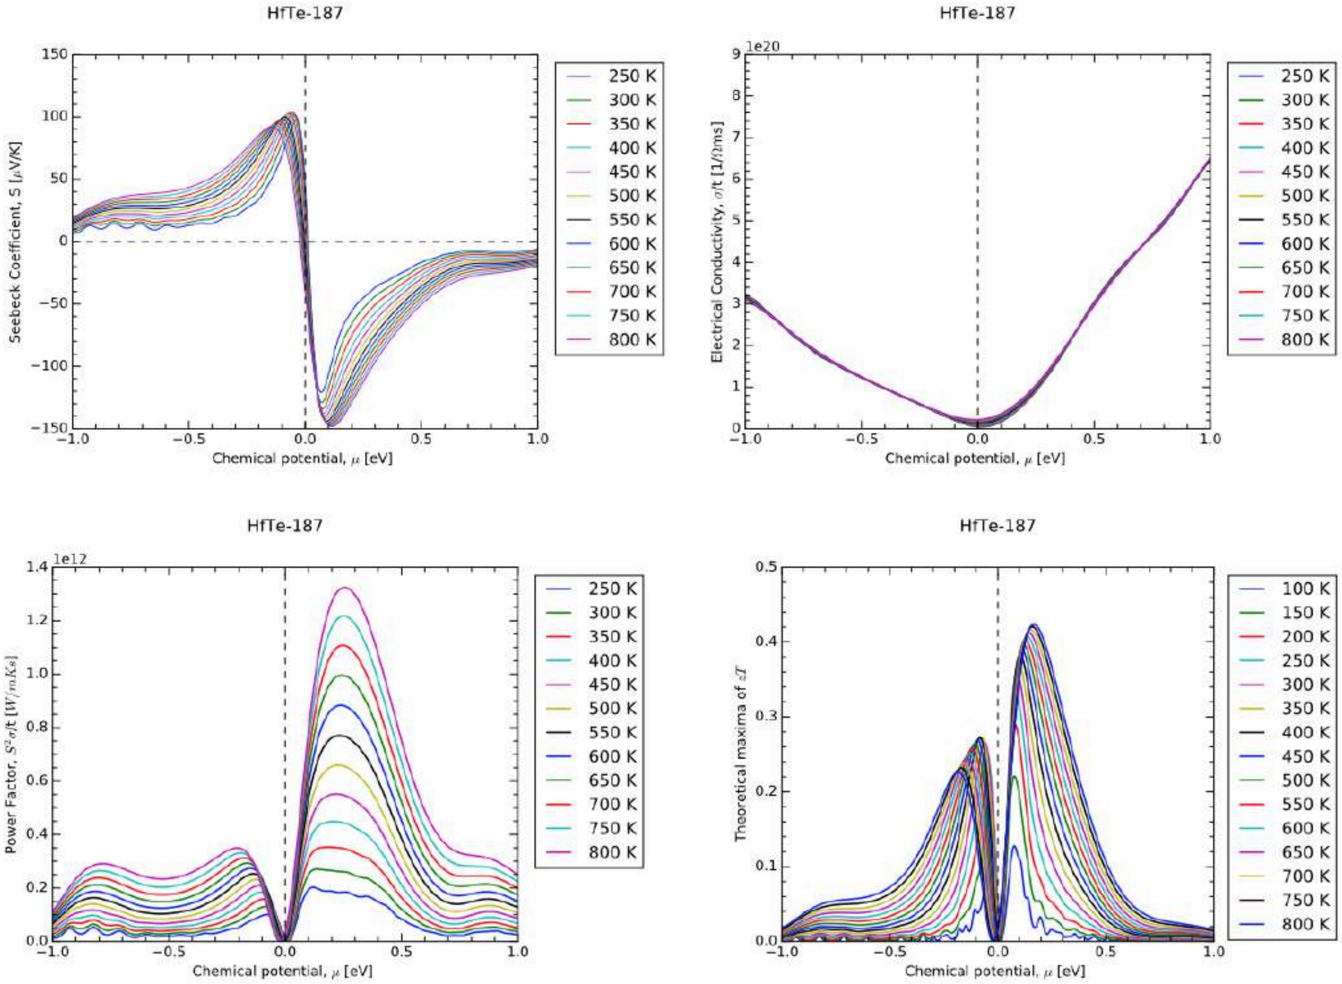


FIG. 34: Thermoelectric properties of HfTe calculated using BoltzTrap code.

## XI. COMPARISON OF THERMAL CONDUCTIVITY IN HfTe AND TiS

Here we compare the total thermal conductivity and its different components in HfTe and TiS, compounds that are predicted to host TDP in their phonon spectra [32].

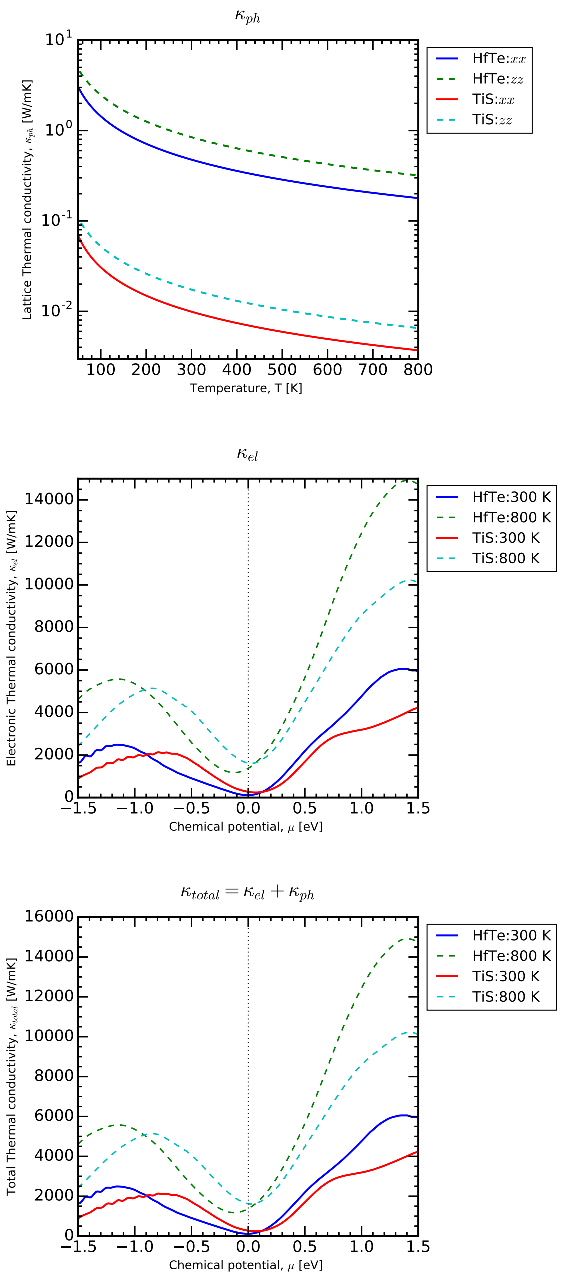


FIG. 35: Comparison of different components of thermal conductivity and total thermal conductivity along different directions in crystal at different temperatures. The $xx$ and $yy$ components of thermal conductivity tensor are same due to the crystal symmetry.

### A. Comparison of Thermoelectric properties

Here we compare the maxima of various thermoelectric properties of TaX obtained for electronic doping case. We also compare the thermoelectric properties of TaX with two other similar compounds predicted by Li et al. [32] - HfTe and TiS. We notice relatively smaller magnitude of thermoelectric effects for hole doping case.

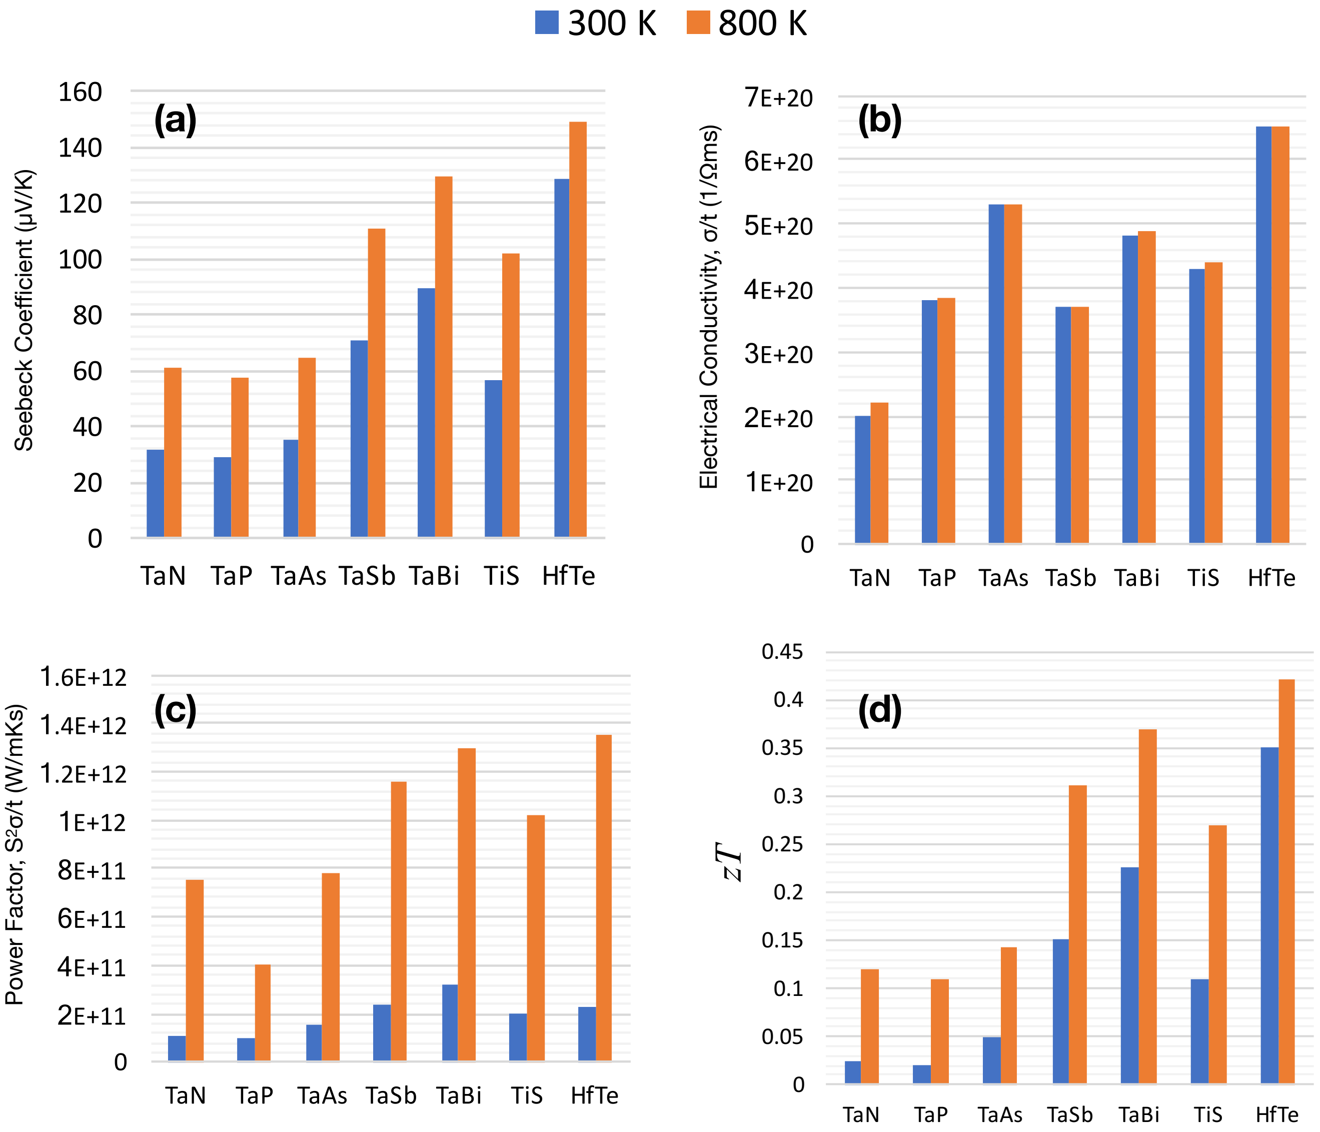


FIG. 36: (Color online) (a) Maximum of Seebeck coefficient or thermopower, (b) maximum of electrical conductivity ($\sigma/t$)obtained at 300 K and 800 K, (c) maximum power factor at 300 K and 800 K, and (d) the theoretical maximum of $zT$. All data is for electron doping case.

## XII. NUMERICAL DETAILS

Density Functional Theory (DFT) based first-principles calculations were carried out using the projector augmented-wave (PAW) method as implemented in the VASP code [12, 13]. We used the PBE exchange-correlation functional as parametrized by Perdew-Burke-Ernzerhof [33]. The SOC was employed by a second-variation method implemented in the VASP code. We considered five valence electrons of Ta ($5d^3 6s^2$) and five valence electrons of Sb ($5s^2 5p^3$) in the PAW pseudo-potential. The lattice parameters were optimized until the Hellmann-Feynman residual forces were less than $10^{-4}$ eV/Å per atom. For convergence of the electronic self-consistent calculations, a total energy difference criterion was defined as $10^{-8}$ eV. We used 600 eV as kinetic energy cutoff of the plane wave basis set and a Γ-type $10 \times 10 \times 10$ $k$-point mesh was employed to optimize the lattice parameters and the self-energy. The phonon calculations were performed for a $2 \times 2 \times 2$ supercell. The PHONOPY code [34] was used for the phonons post-processing, and the PyProcar code [35, 36] was used for the post-processing of electronic bandstructure. SOC was included in the phonon calculations. To verify the stability of the TaSb compound at room temperature, we performed room temperature molecular dynamics (MD) simulations for more than 9800 fs with a time step of 1 fs. The SOC was included in the MD simulations. In MD simulations, we employed a supercell of size $4 \times 4 \times 4$ to guarantee the decay of interatomic force constants within the supercell dimensions. The topological charge of the Weyl points and the surface state spectrum were calculated using the open-source WannierTools code [26]. This code is based on the iterative Green's function mechanism and it performs the post-processing of the Wannier tight binding model hamiltonian obtained from the Wannier90 [37]. We used Ta $s, p, d$, and Sb $s, p$ orbitals as the initial projectors for construction of the Wannier tight binding hamiltonian.

### A. Thermal conductivity and anharmonic high-temperature phonons

To accurately describe the high temperature anharmonicity of TaSb and TaN we used *ab initio* molecular dynamics in combination with the temperature dependent effective potential technique (TDEP) [38–40] to extract effective interatomic force constants at finite temperature. The *ab initio* molecular dynamics simulations were carried out using the PAW method as implemented in VASP [12, 13]. The simulation cell was constructed from a $4 \times 4 \times 4$ repetition of the unit cell (128 atoms). We used a set of seven volumes around equilibrium and ran molecular dynamics at 300K using the Γ-point for Brillouin zone integration and an energy cutoff of 600 eV for about 10000 time steps to ensure good coverage of the phase space. The temperature was controlled with a Nose-Hoover thermostat [41, 42]. A 1.0 femtosecond time step was used in the molecular dynamics (MD) calculations. From the forces obtained from uncorrelated configurations (one every 50 frames), folding into the unit cell is performed and the temperature dependent of the harmonic and anharmonic interatomic force constants are obtained. With this information, we obtain the lattice thermal conductivity.

For the other topological materials, we have used a slightly different approach. We have generated a series of 150 different uncorrelated configurations with a Gaussian distribution around a predefined temperature (lower than the Debye temperature). For each of those configurations, the forces are calculated from first principles and the same methodology described in the previous paragraph was followed. We find a very good convergence of results obtained from 150 uncorrelated configurations and that of obtained from the MD simulations described in the above paragraph.

### B. Details of the thermoelectric properties calculations

We perform the calculation of the thermoelectric properties such as the thermopower or Seebeck coefficient (S), electrical conductivity ($\sigma$), the power factor ($S^2\sigma/\tau$), and the theoretical maximum figure of merit ($zT$). These thermoelectric properties were obtained using the solution of Boltzmann transport equations (BTE) within the constant relaxation time approximation (CRTA) as implemented in the BoltzTrap code [43, 44]. This theory allows us to calculate the Seebeck coefficient tensor independently of the electronic relaxation time ($\tau$) while the electronic conductivity is dependent on $\tau$. The code utilizes the rigid band approximation to change the carrier concentration by rigidly shifting the chemical potential ($\mu$) into valence or conduction bands while the effects of temperature on the electronic bands are neglected. The carrier concentration was considered from range $-1 \times 10^{21}$ to $1 \times 10^{21}$ $cm^{-3}$. The results obtained within the BoltzTrap code have shown very good agreement with experimental measurements, specially for bulk materials [45, 46]. The lattice thermal conductivity evaluated from the TDEP code was used to estimate $zT$. The relaxation time ($\tau$) obtained from the first-principles calculations (electron-phonon interaction) was found to vary in the order of 1 ps with increasing temperature. Therefore, we decided to choose $\tau = 1 \times 10^{-12}$ $s$. However, we observe negligible changes in $zT$ with varying $\tau$ in ps range. This is as expected for systems with small $\kappa_{ph}$ and relatively large $\kappa_{el}$.

---


[1] S. Goedecker, The Journal of Chemical Physics **120**, 9911 (2004).

[2] M. Amsler and S. Goedecker, The Journal of Chemical Physics **133**, 224104 (2010).

[3] F. Jensen, *Introduction to computational chemistry* (John wiley & sons, 2017).

[4] M. Sicher, S. Mohr, and S. Goedecker, The Journal of Chemical Physics **134**, 044106 (2011), https://doi.org/10.1063/1.3530590 .

[5] S. Singh, A. C. Garcia-Castro, I. Valencia-Jaime, F. Muñoz, and A. H. Romero, Phys. Rev. B **94**, 161116 (2016).

[6] S. Singh, W. Ibarra-Hernandez, I. Valencia-Jaime, G. Avendano-Franco, and A. H. Romero, Phys. Chem. Chem. Phys. **18**, 29771 (2016).

[7] O. Pavlic, W. Ibarra-Hernandez, I. Valencia-Jaime, S. Singh, G. Avendaño-Franco, D. Raabe, and A. H. Romero, Journal of Alloys and Compounds **691**, 15 (2017).

[8] J. Murray, J. Taylor, L. Calvert, Y. Wang, E. Gabe, and J. Despault, Journal of the Less Common Metals **46**, 311 (1976).

[9] S.-Y. Xu, I. Belopolski, D. S. Sanchez, C. Zhang, G. Chang, C. Guo, G. Bian, Z. Yuan, H. Lu, T.-R. Chang, P. P. Shibayev, M. L. Prokopovych, N. Alidoust, H. Zheng, C.-C. Lee, S.-M. Huang, R. Sankar, F. Chou, C.-H. Hsu, H.-T. Jeng, A. Bansil, T. Neupert, V. N. Strocov, H. Lin, S. Jia, and M. Z. Hasan, Science Advances **1** (2015), 10.1126/sciadv.1501092.

[10] T. Besara, D. A. Rhodes, K.-W. Chen, S. Das, Q. R. Zhang, J. Sun, B. Zeng, Y. Xin, L. Balicas, R. E. Baumbach, E. Manousakis, D. J. Singh, and T. Siegrist, Phys. Rev. B **93**, 245152 (2016).

[11] Z. K. Liu, L. X. Yang, Y. Sun, T. Zhang, H. Peng, H. F. Yang, C. Chen, Y. Zhang, Y. F. Guo, D. Prabhakaran, M. Schmidt, Z. Hussain, S. K. Mo, C. Felser, B. Yan, and Y. L. Chen, Nat Mater **15**, 27 (2016).

[12] G. Kresse and J. Furthmüller, Phys. Rev. B **54**, 11169 (1996).

[13] G. Kresse and D. Joubert, Phys. Rev. B **59**, 1758 (1999).

[14] Z.-j. Wu, E.-j. Zhao, H.-p. Xiang, X.-f. Hao, X.-j. Liu, and J. Meng, Phys. Rev. B **76**, 054115 (2007).

[15] S. Singh, I. Valencia-Jaime, O. Pavlic, and A. H. Romero, Phys. Rev. B **97**, 054108 (2018).

[16] Born, Max and Huang, Kun, *Dynamical theory of crystal lattices* (Oxford, Clarendon Press, 1954).

[17] D. Shi, B. Wen, R. Melnik, S. Yao, and T. Li, Journal of Solid State Chemistry **182**, 2664 (2009).

[18] R. Hill, Proceedings of the Physical Society. Section A **65**, 349 (1952).

[19] S. Pugh, Philosophical Magazine Series 7 **45**, 823 (1954).

[20] B. Q. Lv, H. M. Weng, B. B. Fu, X. P. Wang, H. Miao, J. Ma, P. Richard, X. C. Huang, L. X. Zhao, G. F. Chen, Z. Fang, X. Dai, T. Qian, and H. Ding, Phys. Rev. X **5**, 031013 (2015).

[21] S.-Y. Xu, I. Belopolski, N. Alidoust, M. Neupane, G. Bian, C. Zhang, R. Sankar, G. Chang, Z. Yuan, C.-C. Lee, S.-M. Huang, H. Zheng, J. Ma, D. S. Sanchez, B. Wang, A. Bansil, F. Chou, P. P. Shibayev, H. Lin, S. Jia, and M. Z. Hasan, Science **349**, 613 (2015).

[22] L. Lu, Z. Wang, D. Ye, L. Ran, L. Fu, J. D. Joannopoulos, and M. Soljačić, Science **349**, 622 (2015).

[23] Z. Zhu, G. W. Winkler, Q. Wu, J. Li, and A. A. Soluyanov, Phys. Rev. X **6**, 031003 (2016).

[24] B. Q. Lv, Z. L. Feng, Q. N. Xu, X. Gao, J. Z. Ma, L. Y. Kong, P. Richard, Y. B. Huang, V. N. Strocov, C. Fang, H. M. Weng, Y. G. Shi, T. Qian, and H. Ding, Nature **546**, 627 (2017).

[25] H. Weng, C. Fang, Z. Fang, and X. Dai, Phys. Rev. B **94**, 165201 (2016).

[26] Q. Wu, S. Zhang, H.-F. Song, M. Troyer, and A. A. Soluyanov, Computer Physics Communications **224**, 405 (2018).

[27] D. Gresch, G. Autès, O. V. Yazyev, M. Troyer, D. Vanderbilt, B. A. Bernevig, and A. A. Soluyanov, Phys. Rev. B **95**, 075146 (2017).

[28] A. A. Soluyanov, D. Gresch, Z. Wang, Q. Wu, M. Troyer, X. Dai, and B. A. Bernevig, Nature **527**, 495 (2015).

[29] X. Wan, A. M. Turner, A. Vishwanath, and S. Y. Savrasov, Phys. Rev. B **83**, 205101 (2011).

[30] N. Marzari and D. Vanderbilt, Phys. Rev. B **56**, 12847 (1997).

[31] I. Souza, N. Marzari, and D. Vanderbilt, Phys. Rev. B **65**, 035109 (2001).

[32] J. Li, Q. Xie, S. Ullah, R. Li, H. Ma, D. Li, Y. Li, and X.-Q. Chen, Phys. Rev. B **97**, 054305 (2018).

[33] J. P. Perdew, K. Burke, and M. Ernzerhof, Phys. Rev. Lett. **77**, 3865 (1996).

[34] A. Togo, F. Oba, and I. Tanaka, Phys. Rev. B **78**, 134106 (2008).

[35] A. H. Romero and F. Munoz, "Pyprocar code," (2015).

[36] S. Singh and A. H. Romero, Phys. Rev. B **95**, 165444 (2017).

[37] A. A. Mostofi, J. R. Yates, Y.-S. Lee, I. Souza, D. Vanderbilt, and N. Marzari, Computer Physics Communications **178**, 685 (2008).

[38] O. Hellman, I. A. Abrikosov, and S. I. Simak, Physical Review B **84**, 180301 (2011).

[39] O. Hellman, P. Steneteg, I. A. Abrikosov, and S. I. Simak, Physical Review B **87**, 104111 (2013).

[40] A. H. Romero, E. K. U. Gross, M. J. Verstraete, and O. Hellman, Physical Review B **91** (2015).

[41] S. Nosé, Molecular physics **52**, 255 (1984).

[42] W. G. Hoover, Physical Review A **31**, 1695 (1985).

[43] G. K. H. Madsen and D. J. Singh, Computer Physics Communications **175**, 67 (2006), arXiv:cond-mat/0602203 .

[44] T. J. Scheidemantel, C. Ambrosch-Draxl, T. Thonhauser, J. V. Badding, and J. O. Sofo, Phys. Rev. B **68**, 125210 (2003).

[45] D. J. Singh, Phys. Rev. B **81**, 195217 (2010).

[46] T. Thonhauser, T. J. Scheidemantel, J. O. Sofo, J. V. Badding, and G. D. Mahan, Phys. Rev. B **68**, 085201 (2003).
